# Supplementary material for: Pose-NDF: Modeling Human Pose Manifolds with Neural Distance Fields
Source: arXiv:2207.13807 source file (2022-07-27)
Supplement: Supplementary file 1 [file network.tex]

\subsection{Data Preparation}
\label{sec:suppl_data_prep}

\noindent\textbf{Training data:} We use the AMASS dataset~\cite{AMASS:2019} to train our model. We assume that AMASS represents a dataset of realisitc poses and all the poses, which are not part of AMASS are not plausible, with some confidence value. As mentioned in the experiment section, we prepare a dataset of points (poses) and corresponding distance values using kNN. We implement kNN using FAISS~\cite{johnson2019billion} and Pytorch3D~\cite{ravi2020pytorch3d}. We first approximate $k'$-NN of a query pose using FAISS and L2 distances, where $k' >> k$. Then we use the geodesic distance to find exact $k$ neighbours from these $k'$ neighbours. Specifically we use $k' = 500$ and $k =5 $ in our case. We use this multi-step approach, because the AMASS dataset is very large and our proposed data preparation steps are efficient. We generate the ground truth distance by taking the average of the $k$ smallest distances. We use approximately 21M poses from the AMASS dataset for data preparation and training. Following VPoser~\cite{SMPL-X:2019}, we also sample random frames from the motion sequence data, in order to avoid repetitive poses.

\noindent\textbf{Evaluation and Validation:} For validation, we use the validation split of the AMASS dataset and prepare distance values with respect to the train split. For testing the accuracy of the distance field prediction in our model, we use the test-split of AMASS dataset. For downstream tasks, we use existing real world mocap data like~\cite{HPS} and~\cite{AMASS:2019}.
% For image based 3d pose estimation, we use existing EHF dataset, which also includes ground truth SMPL parameters, 3DPW~\cite{vonMarcard2018}, MS-COCO~\cite{lin2014microsoft} and LSP~\cite{Johnson10} dataset. 
For comparison on the EHF dataset, we follow the evaluation provided in~\cite{SMPL-X:2019}, \ie we align the predicted SMPL mesh with the ground truth using Procrustes and then calculate the error on SMPL vertices (not on face and hands).

\subsection{Network Architecture}
\label{sec:suppl_net}
We implement the hierarchical pose encoding network using  structural MLPs~\cite{LEAP:CVPR:21,Aksan_2019_ICCV}, where each MLP consists of 2 layers, followed by a 5 layer MLP for distance field prediction. We use softplus as activation for the hidden layers, with $\beta = 100$. 
