# Supplementary material for: Pose-NDF: Modeling Human Pose Manifolds with Neural Distance Fields
Source: arXiv:2207.13807 source file (2022-07-27)
Supplement: Supplementary file 2 [file results.tex]

\subsection{Motion Denoising}
\label{sec:suppl_motion_denoise}

We show more results of motion denoising in Fig~\ref{fig:denoise_suppl}. We observe that the VPoser based motion denoising does not change the pose much if the noisy observation seems similar to common poses like standing with hands near the body (first row in Fig~\ref{fig:denoise_suppl}) and changes significantly in a random way when the poses look rare (bottom row in Fig~\ref{fig:denoise_suppl}). HuMoR changes the pose into m ore realistic poses at first (for initial frames), but results in unrealistic poses later because of accumulation of changes over time, \eg (bottom-left in Fig~\ref{fig:denoise_suppl}). \blah{} seems to perform better in all such cases, resulting in realistic poses and also is not deviating much from noisy observations.

\begin{figure}[t]
	\centering
	\begin{tabular}{ c |c}
				\begin{overpic}[width=0.48\textwidth,unit=1mm]{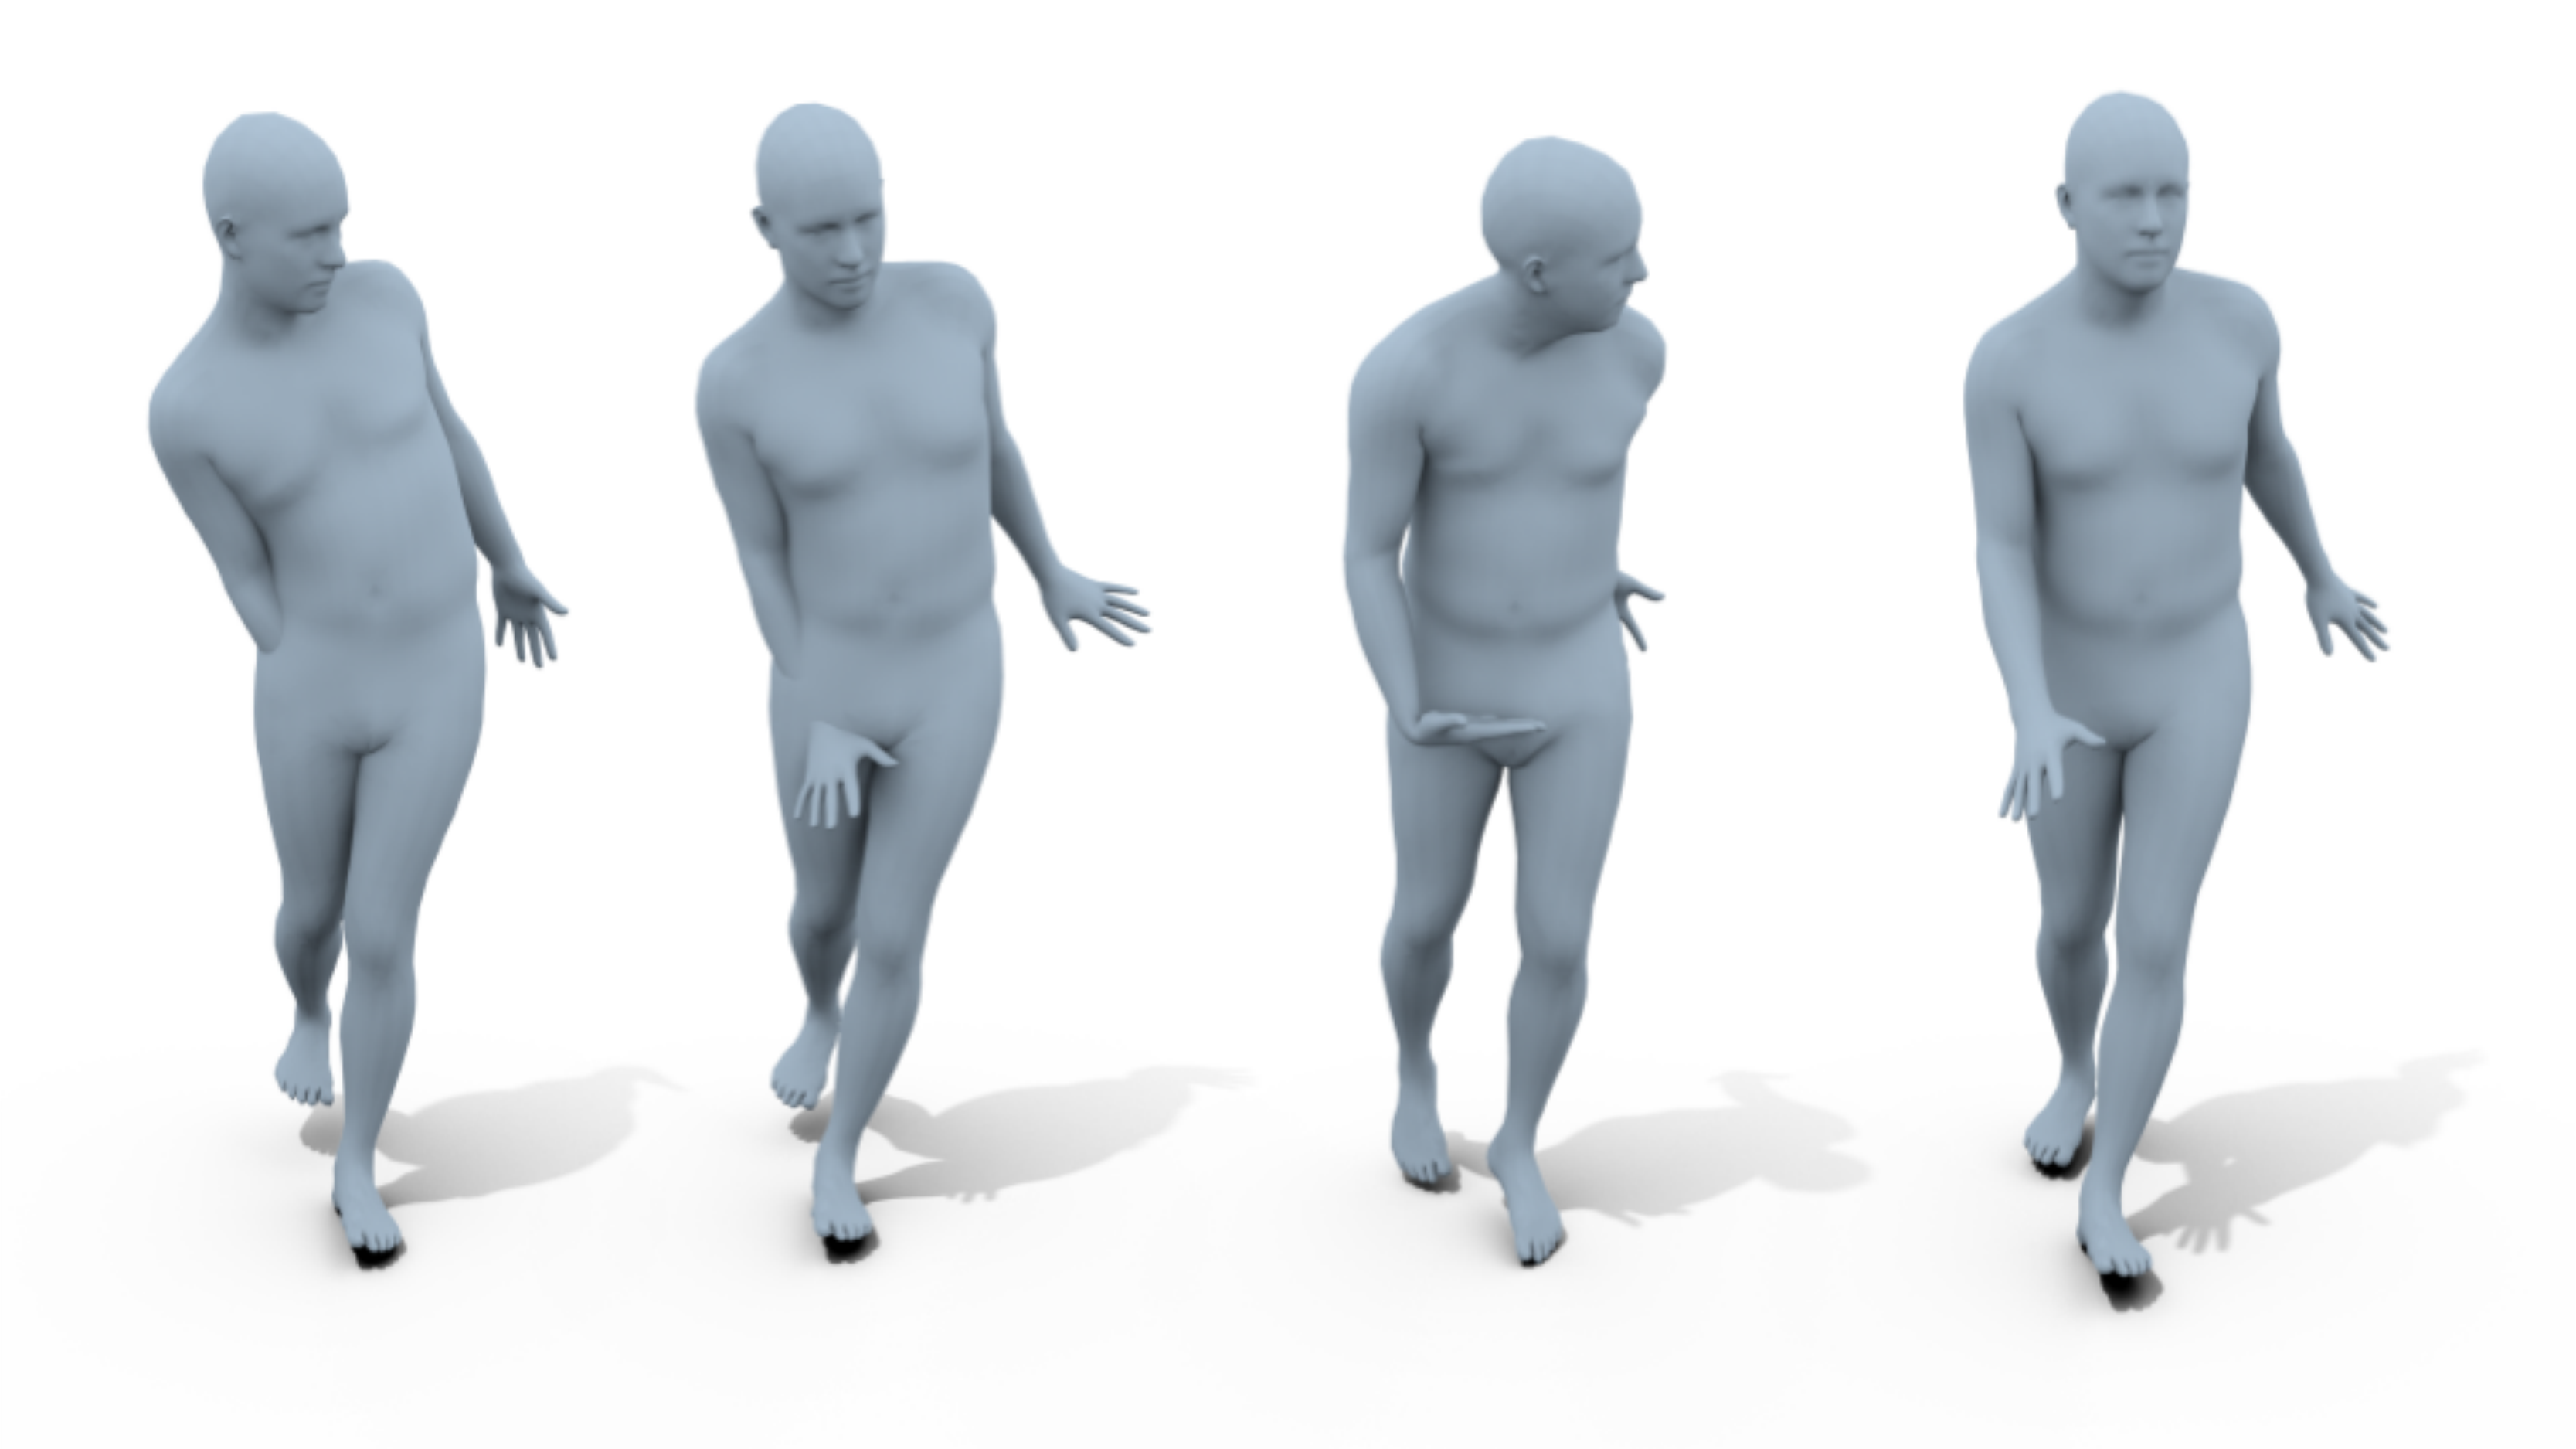}
     		\put(3,32){\colorbox{white}{\parbox{0.05\linewidth}{%
     \scriptsize{Input}}}}
          		\put(13,32){\colorbox{white}{\parbox{0.05\linewidth}{%
     \scriptsize{VPoser}}}}
  	    \put(28,32){\colorbox{white}{\parbox{0.05\linewidth}{%
     \scriptsize{HuMoR}}}}
       	    \put(45,32){\colorbox{white}{\parbox{0.05\linewidth}{%
     \scriptsize{Ours}}}}

\end{overpic}
&
				\begin{overpic}[width=0.48\textwidth,unit=1mm]{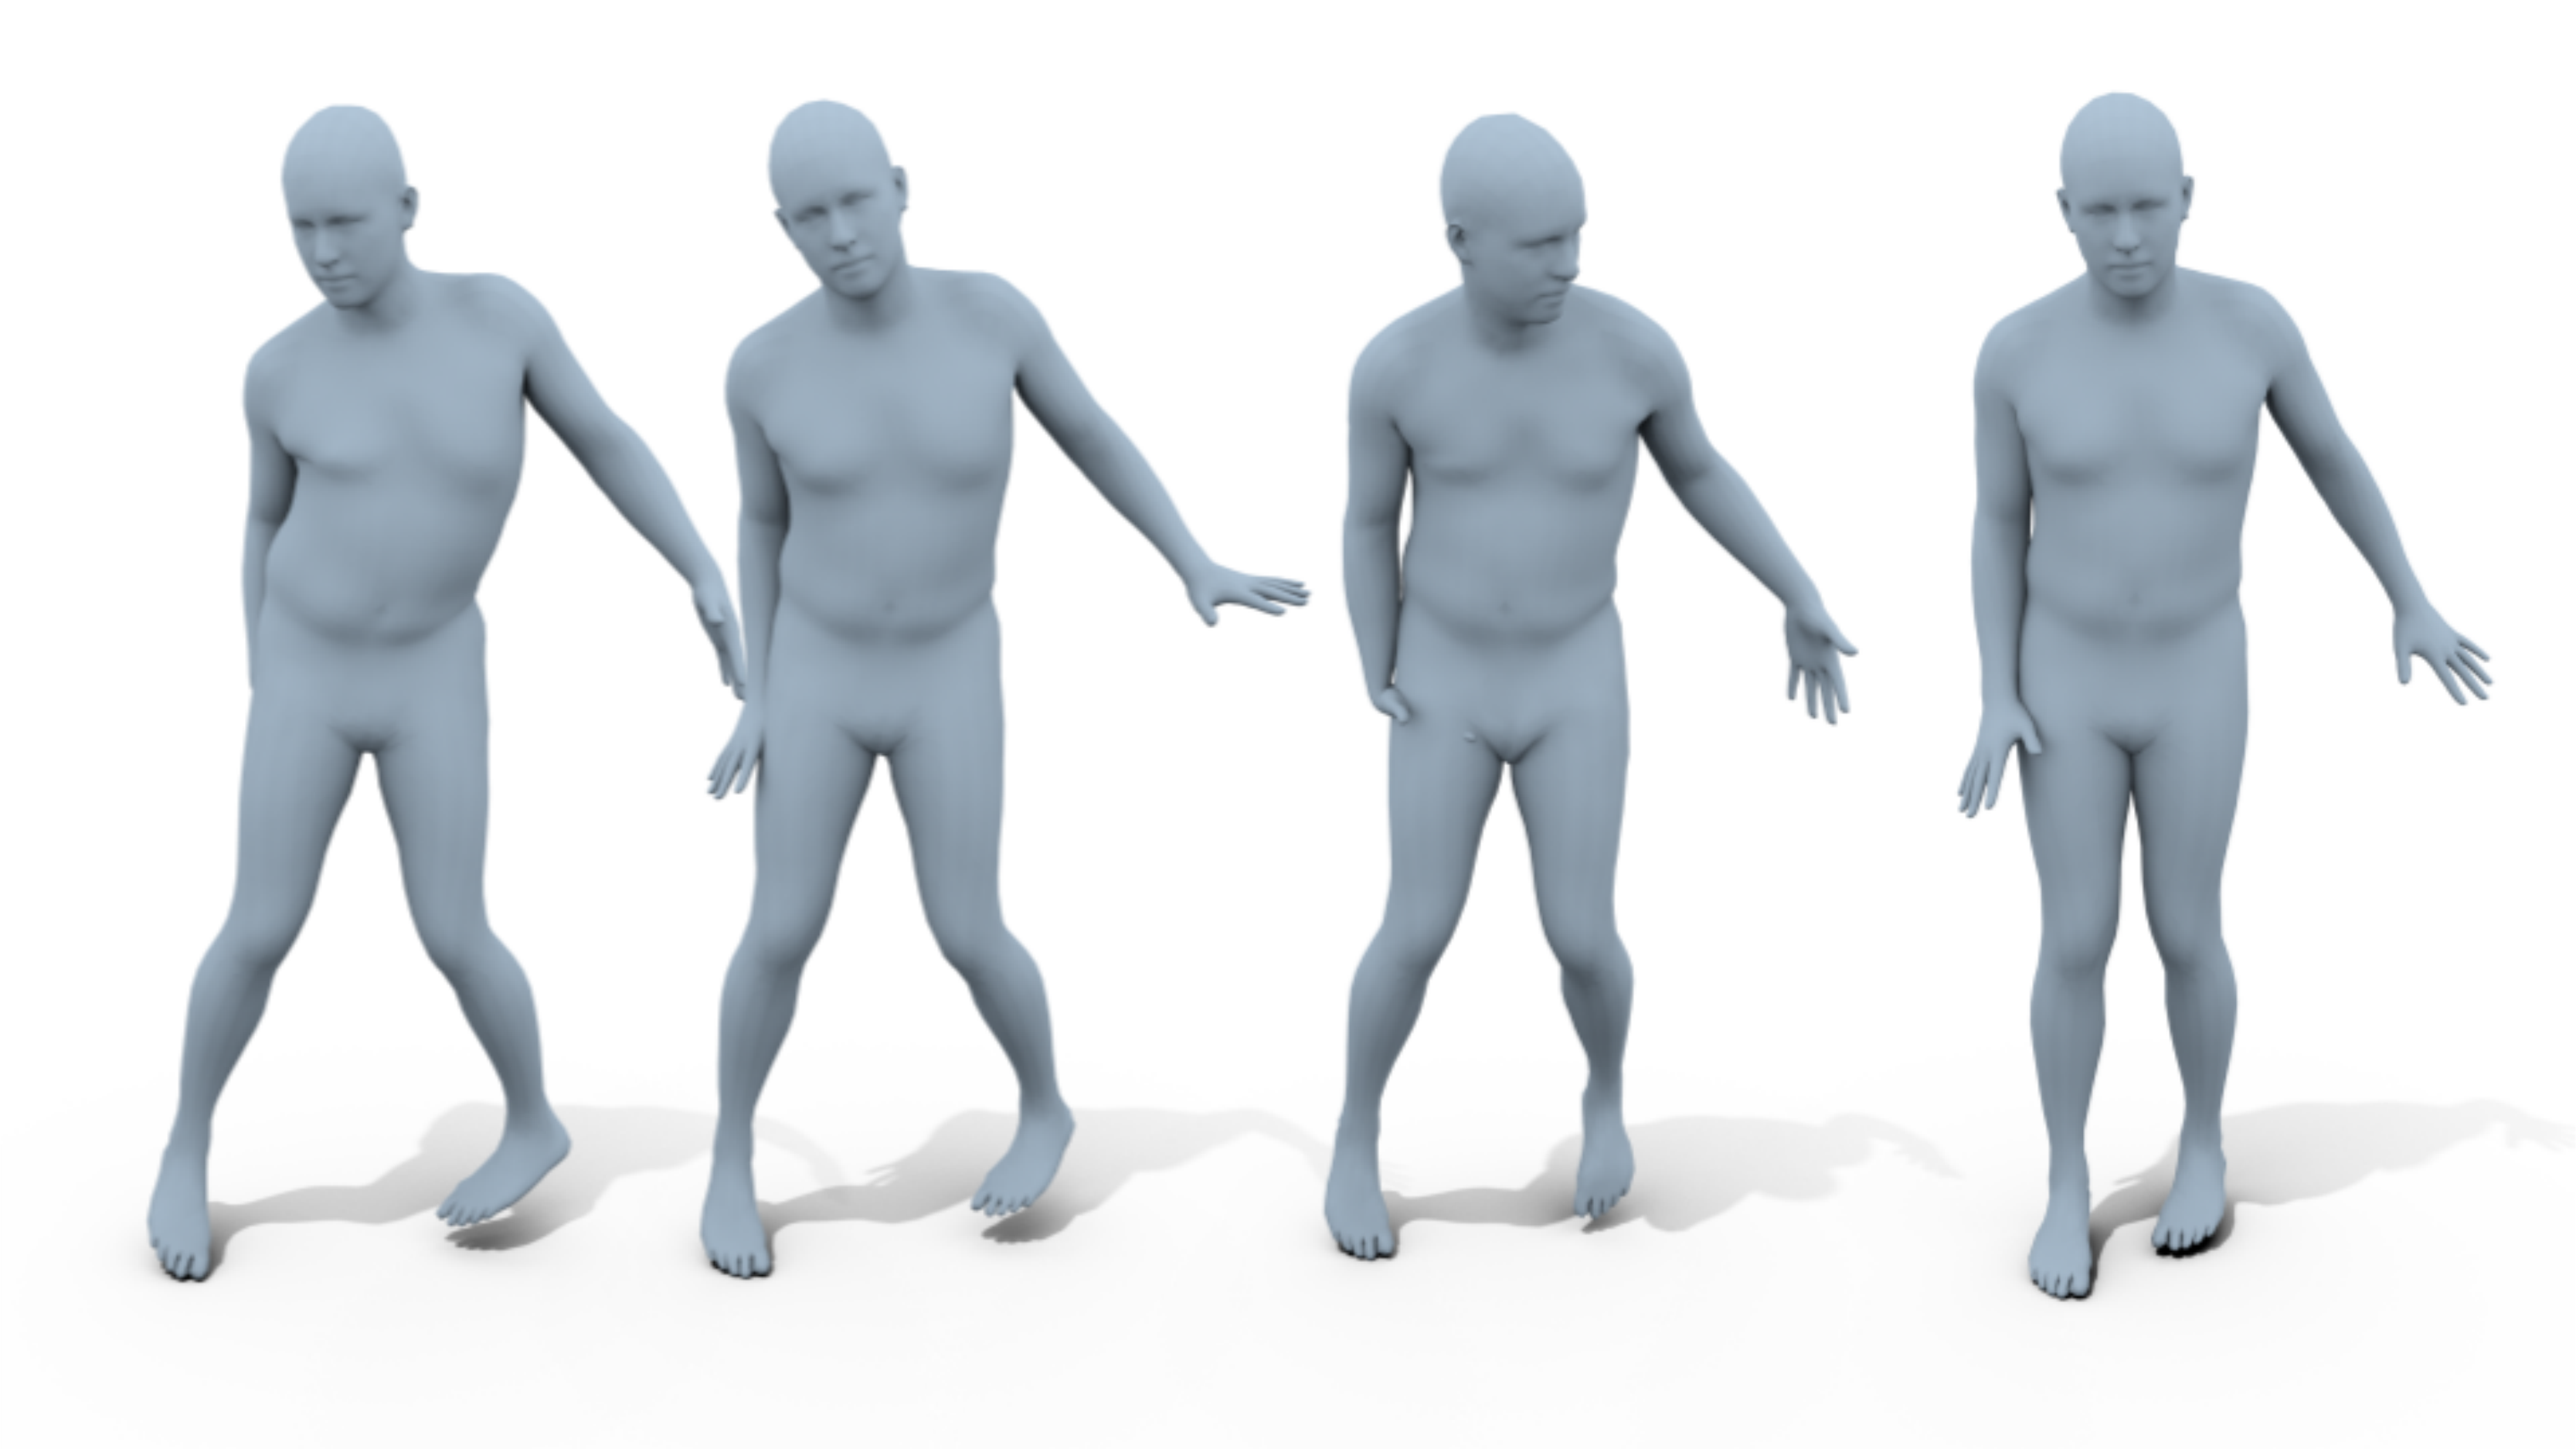}
     		\put(3,32){\colorbox{white}{\parbox{0.05\linewidth}{%
     \scriptsize{Input}}}}
          		\put(13,32){\colorbox{white}{\parbox{0.05\linewidth}{%
     \scriptsize{VPoser}}}}
  	    \put(28,32){\colorbox{white}{\parbox{0.05\linewidth}{%
     \scriptsize{HuMoR}}}}
       	    \put(45,32){\colorbox{white}{\parbox{0.05\linewidth}{%
     \scriptsize{Ours}}}}

\end{overpic}
\end{tabular}
	\begin{tabular}{ c |c}
				\begin{overpic}[width=0.48\textwidth,unit=1mm]{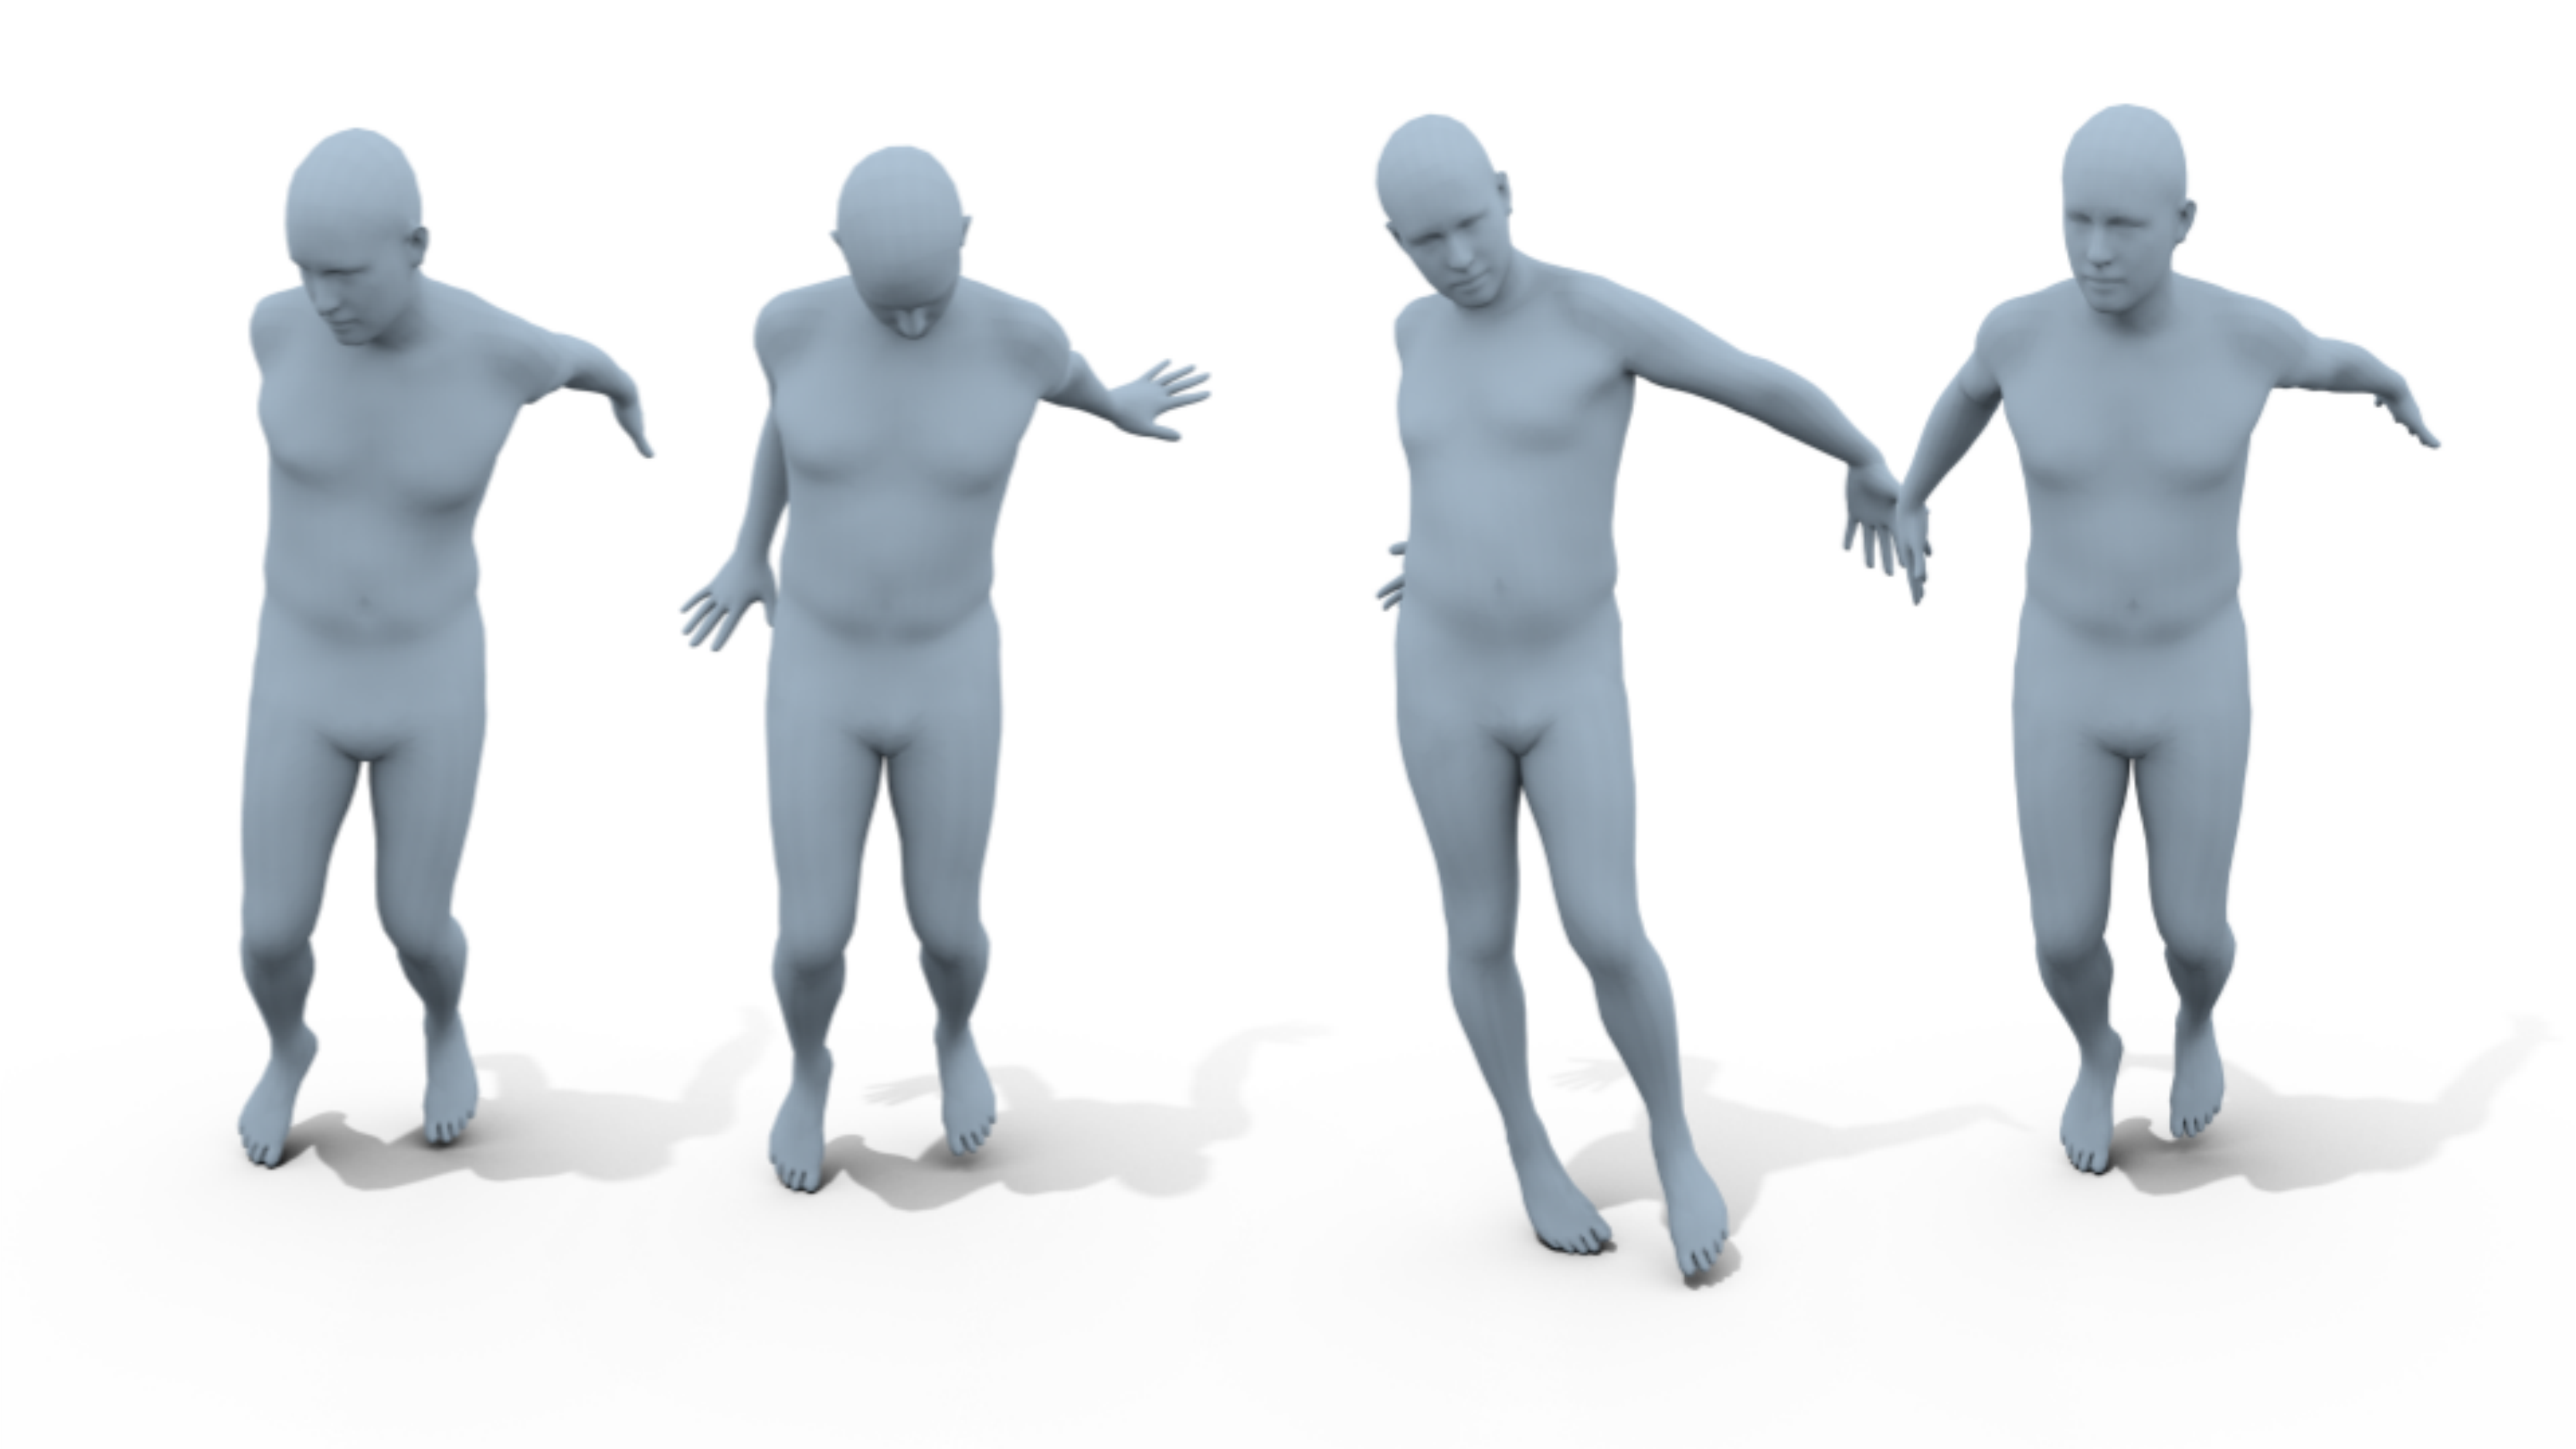}
     		\put(3,32){\colorbox{white}{\parbox{0.05\linewidth}{%
     \scriptsize{Input}}}}
          		\put(13,32){\colorbox{white}{\parbox{0.05\linewidth}{%
     \scriptsize{VPoser}}}}
  	    \put(28,32){\colorbox{white}{\parbox{0.05\linewidth}{%
     \scriptsize{HuMoR}}}}
       	    \put(45,32){\colorbox{white}{\parbox{0.05\linewidth}{%
     \scriptsize{Ours}}}}

\end{overpic}
&
				\begin{overpic}[width=0.48\textwidth,unit=1mm]{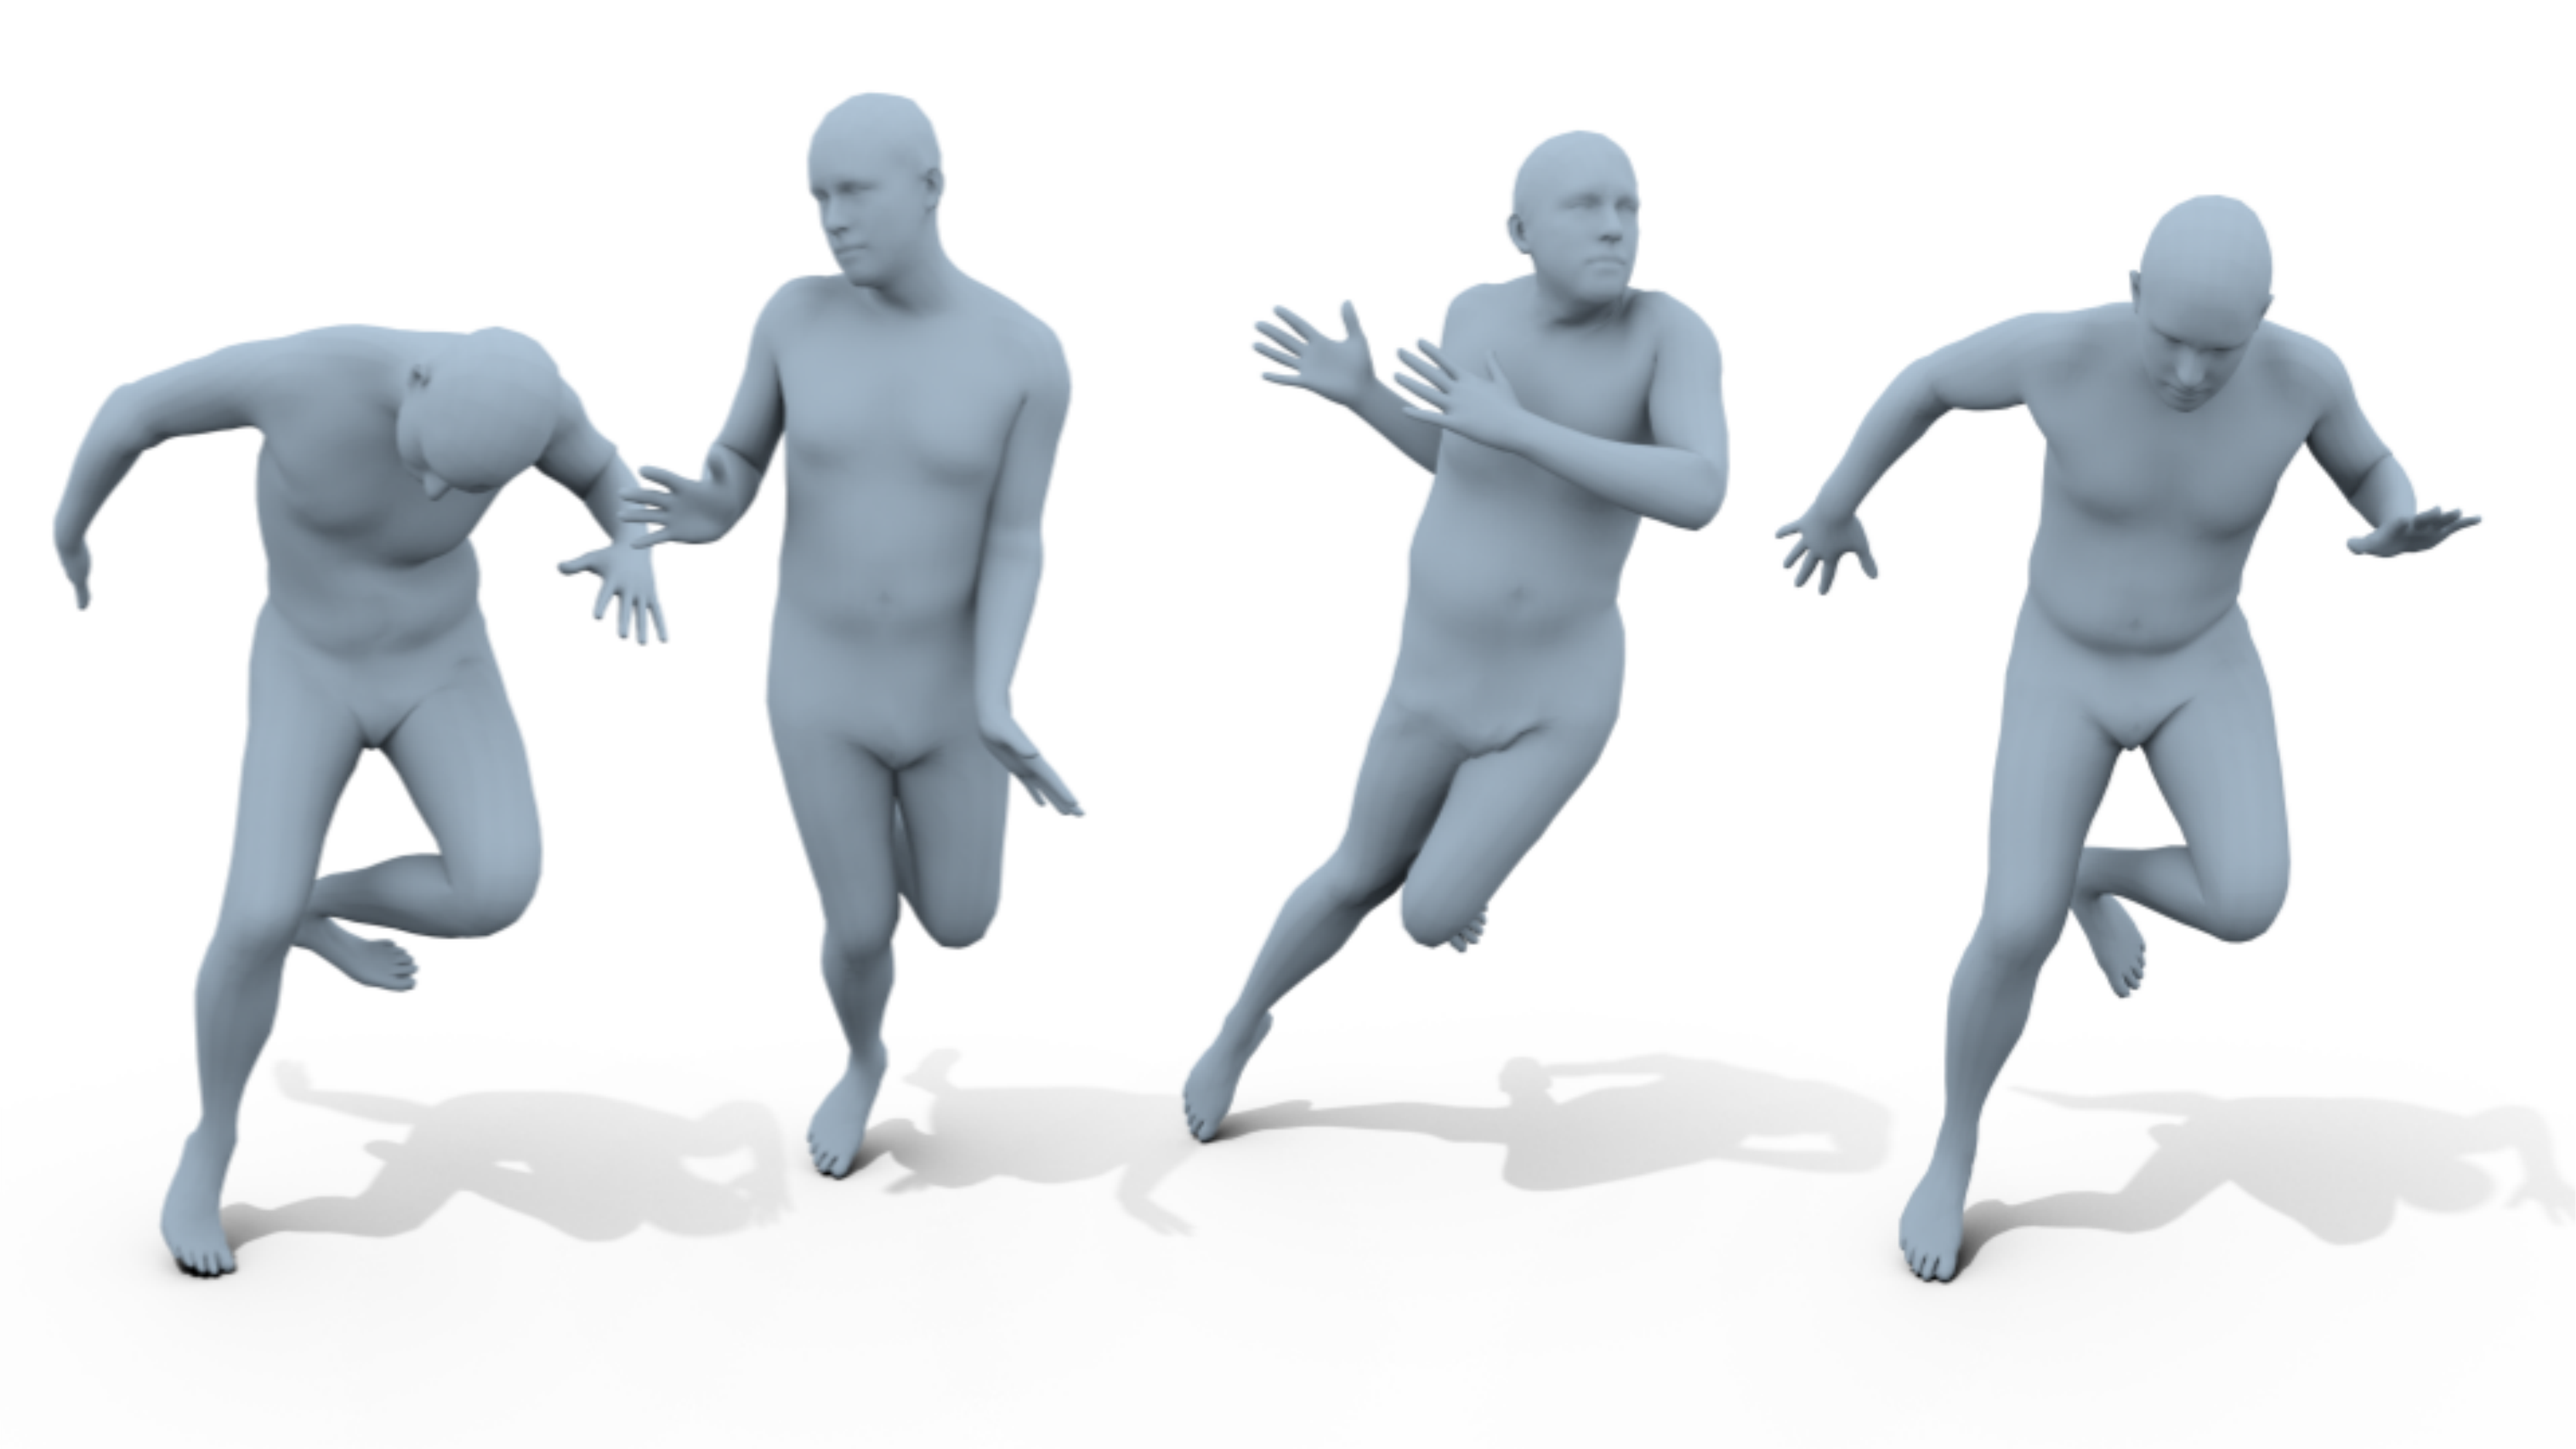}
     		\put(3,32){\colorbox{white}{\parbox{0.05\linewidth}{%
     \scriptsize{Input}}}}
          		\put(13,32){\colorbox{white}{\parbox{0.05\linewidth}{%
     \scriptsize{VPoser}}}}
  	    \put(28,32){\colorbox{white}{\parbox{0.05\linewidth}{%
     \scriptsize{HuMoR}}}}
       	    \put(45,32){\colorbox{white}{\parbox{0.05\linewidth}{%
     \scriptsize{Ours}}}}

\end{overpic}
\end{tabular}
	\caption{\textbf{Motion denoising} for noisy mocap data (``Noissy AMASS''). We observe that \blah{} based motion denoising makes the pose realistic and also resembles the input observation, while VPoser and HuMoR still result in unrealistic poses and in some cases deviate too much from the input observation (bottom-left) }
	\label{fig:denoise_suppl}
 	%\vspace{-0.5cm}
\end{figure}

We evaluate the average \% of self-intersecting mesh faces in the motion denoising task to evaluate which method produces more realistic poses. As seen from qualitative examples, HuMoR and VPoser generate results with self-intersecting poses. We evaluated this quantitatively, by counting the number of intersecting faces for all methods in Table~\ref{tab:intersection}. \blah{} clearly produces less intersections, which we credit to our detailed manifold.

\begin{table}[t]
\setlength{\tabcolsep}{1.0em}
\centering
\caption{Average \% of self-intersecting mesh faces in motion denoising. It can be seen that in most cases, \blah{} produces less intersections than VPoser and HuMoR. } 
\resizebox{\textwidth}{!}{
\begin{tabular}{lcccc}
\toprule
\diagbox{Method}{Data} & HPS & AMASS & Noisy AMASS & Partial Observation\\
\midrule
Input                       & 3.13 & 1.14 & 2.54  &  -   \\
VPoser~\cite{SMPL-X:2019}  &  3.16 & 1.36 & 2.54  &  2.98   \\
HuMoR~\cite{rempe2021humor} &  2.81 & \textbf{1.04} &  1.43  &  2.13  \\
\textbf{\blah{}}         &  \textbf{2.28} & 1.05 & \textbf{1.40}  &  \textbf{2.01} \\
\bottomrule
\end{tabular}
\label{tab:intersection}
}

\end{table}

\subsection{Fitting to partial data}
\label{sec:suppl_partial}

We show qualitative results of estimating 3D poses from partial observations. As discussed we perform this experiment on three different kinds of occlusions, namely 1) occluded left leg, 2) occluded left arm and 3) occluded right shoulder and upper arm. We observe that VPoser is biased towards mean poses, (\eg as seen in Fig.~\ref{fig:partial_suppl}), VPoser tends to produce nearly straight legs for occluded leg cases, which is more commonly seen in training data. On the other hand HuMoR and PoseNDF produce more variety, but in some cases of HuMoR, the resulting pose looks unrealistic due to accumulation in correction in input pose. For our method, it highly depends on initialization. Since we initialise randomly near the mean pose in our experiments, it looks similar to VPoser in most cases.

% Since we have used an initialization close to rest position, our optimization method generates smaller error for occluded legs but higher errors for occluded arms and shoulders, as they usually are more far away from the rest pose. 
% % For HuMoR, the motion generated is realistic and plausible, but in some cases results in large deviation from ground truth, \eg in Fig.~\ref{fig:partial_amass} (col. 1). This is because the person bends his leg in this motion and then straightens it abruptly. It can be seen that HuMoR continues to move along the same pose direction, which results in an unrealistic pose.  
% For HuMoR, the motion generated is realistic and plausible, but in some cases results in large deviation from ground truth, because of accumulation in correction in input pose. 

\begin{figure}[t]
	\centering
	\begin{tabular}{ c |c}
				\begin{overpic}[width=0.48\textwidth,unit=1mm]{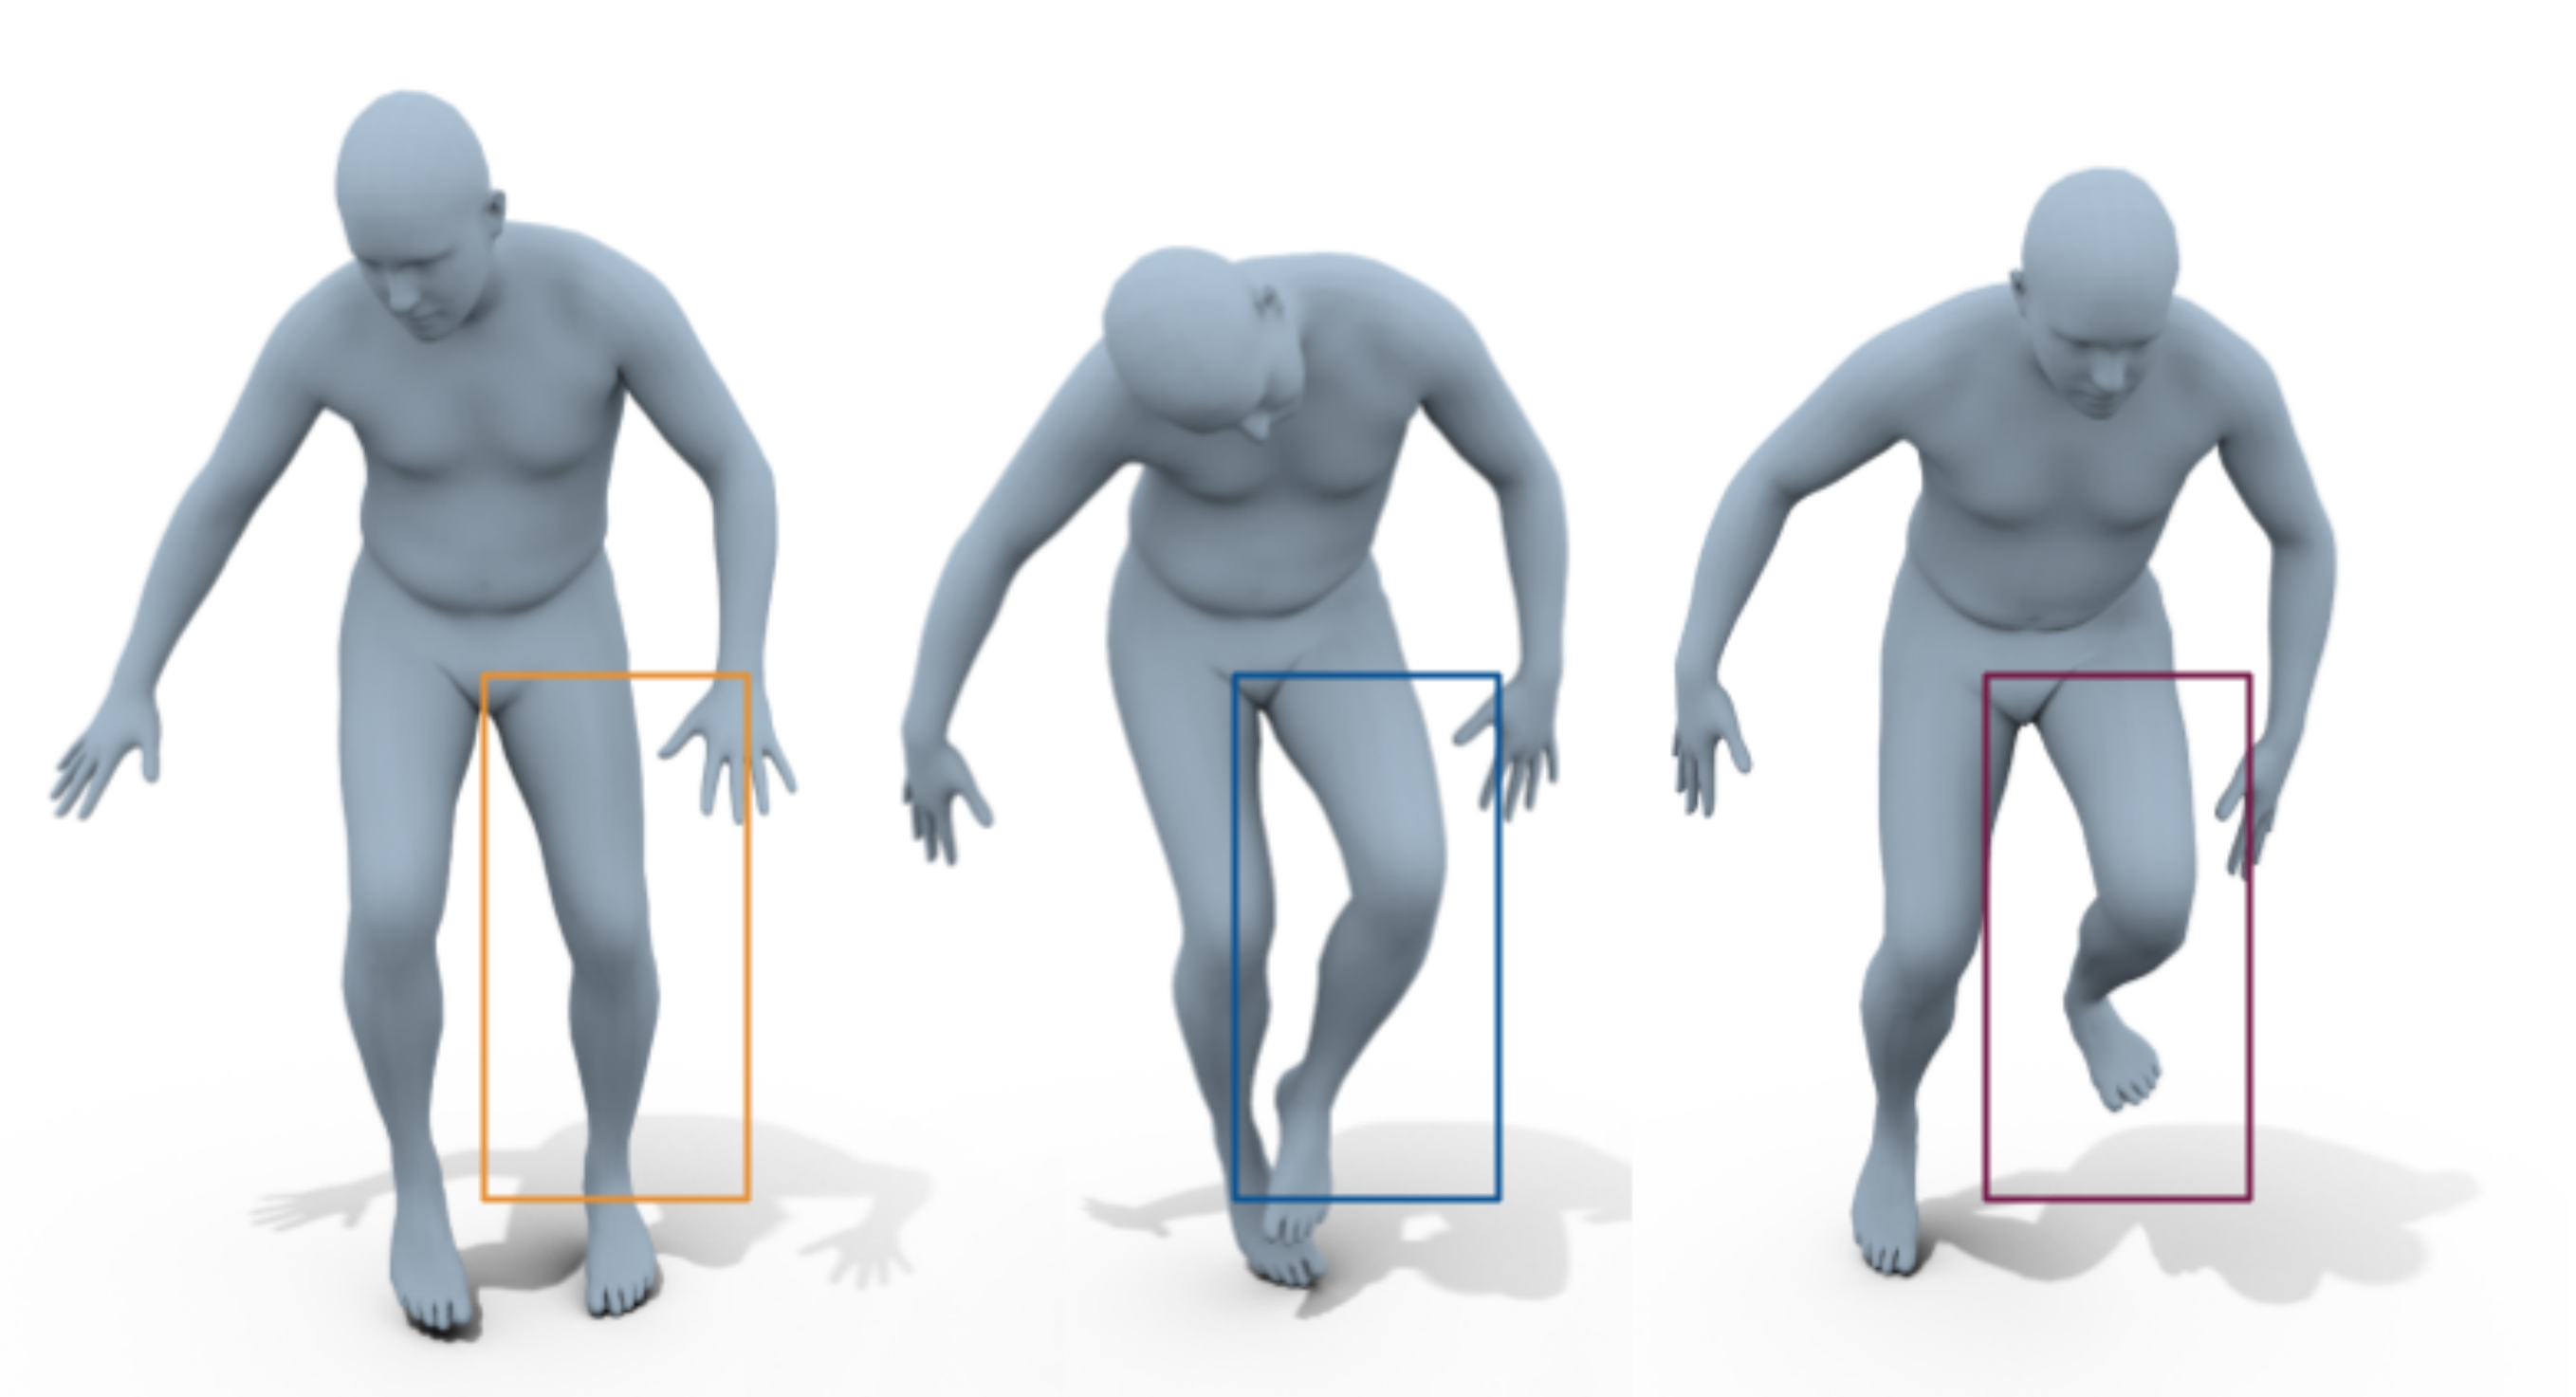}
    %  		\put(5,32){\colorbox{white}{\parbox{0.05\linewidth}{%
    %  \scriptsize{VPoser}}}}

  	 %   \put(25,32){\colorbox{white}{\parbox{0.05\linewidth}{%
    %  \scriptsize{HuMoR}}}}
    %   	    \put(42,32){\colorbox{white}{\parbox{0.05\linewidth}{%
    %  \scriptsize{Ours}}}}

\end{overpic}
&
				\begin{overpic}[width=0.48\textwidth,unit=1mm]{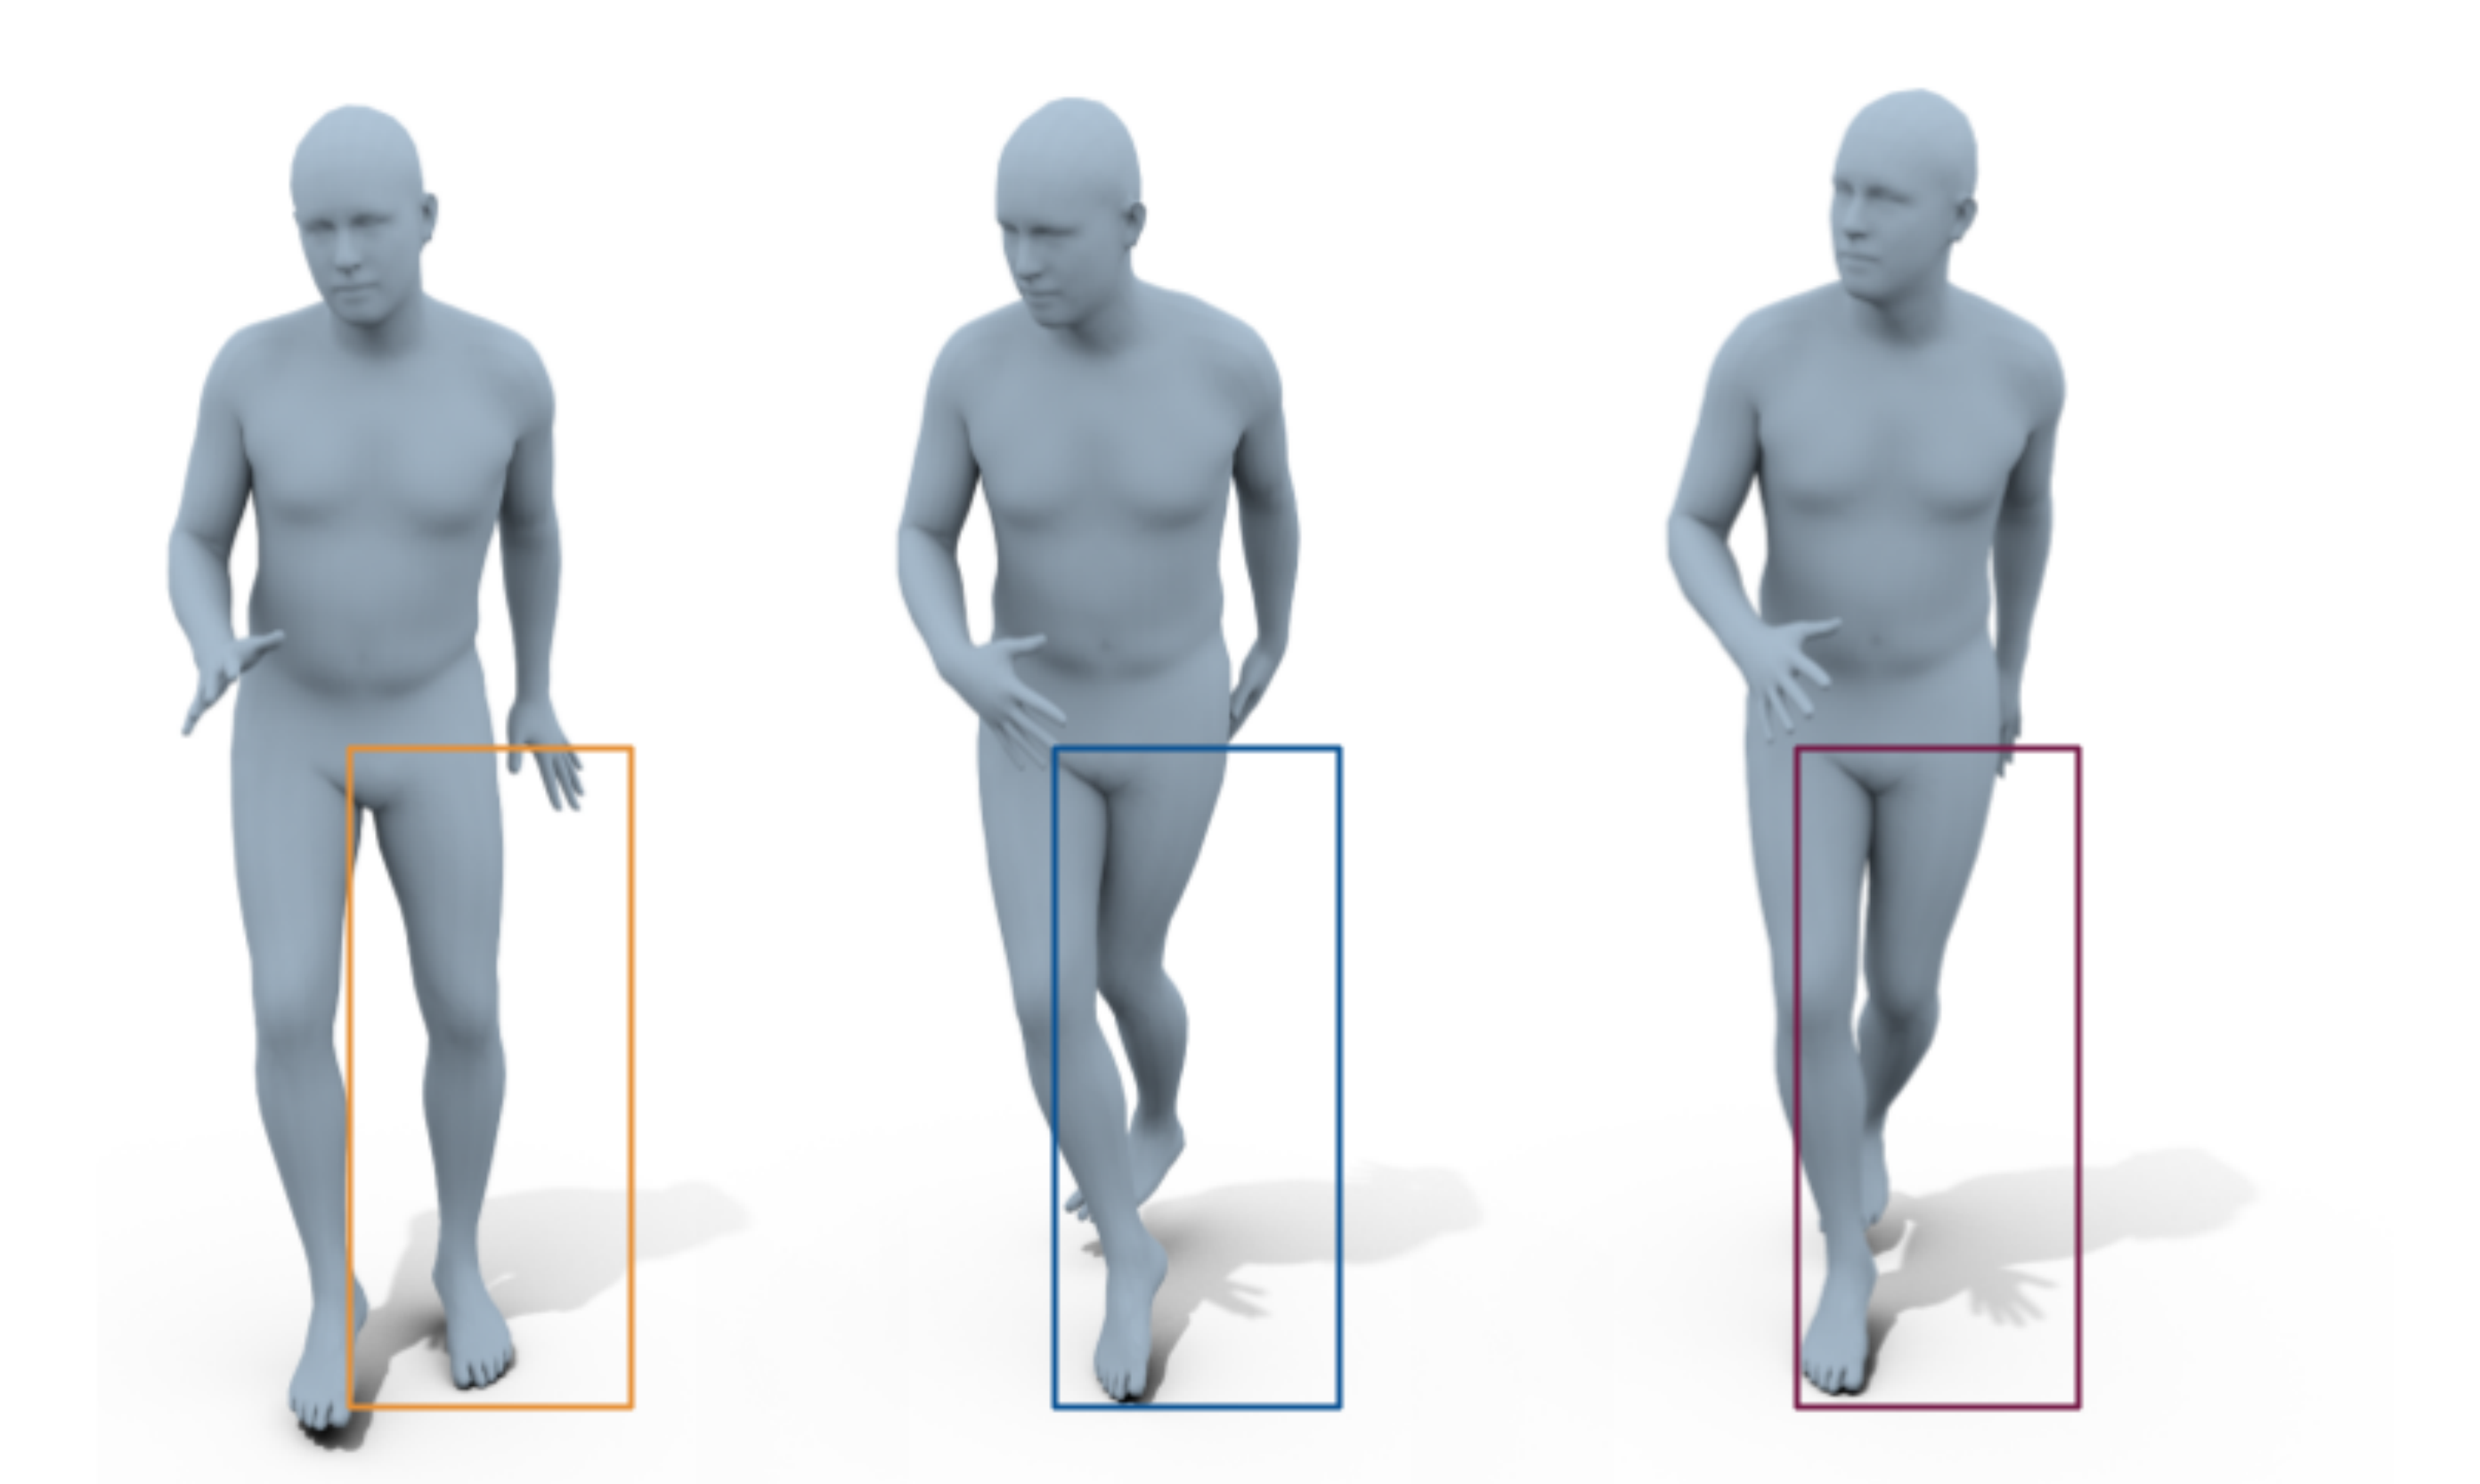}
    %  		\put(5,32){\colorbox{white}{\parbox{0.05\linewidth}{%
    %  \scriptsize{VPoser}}}}

  	 %   \put(25,32){\colorbox{white}{\parbox{0.05\linewidth}{%
    %  \scriptsize{HuMoR}}}}
    %   	    \put(42,32){\colorbox{white}{\parbox{0.05\linewidth}{%
    %  \scriptsize{Ours}}}}

\end{overpic}
\end{tabular}
\begin{tabular}{ c |c}
				\begin{overpic}[width=0.48\textwidth,unit=1mm]{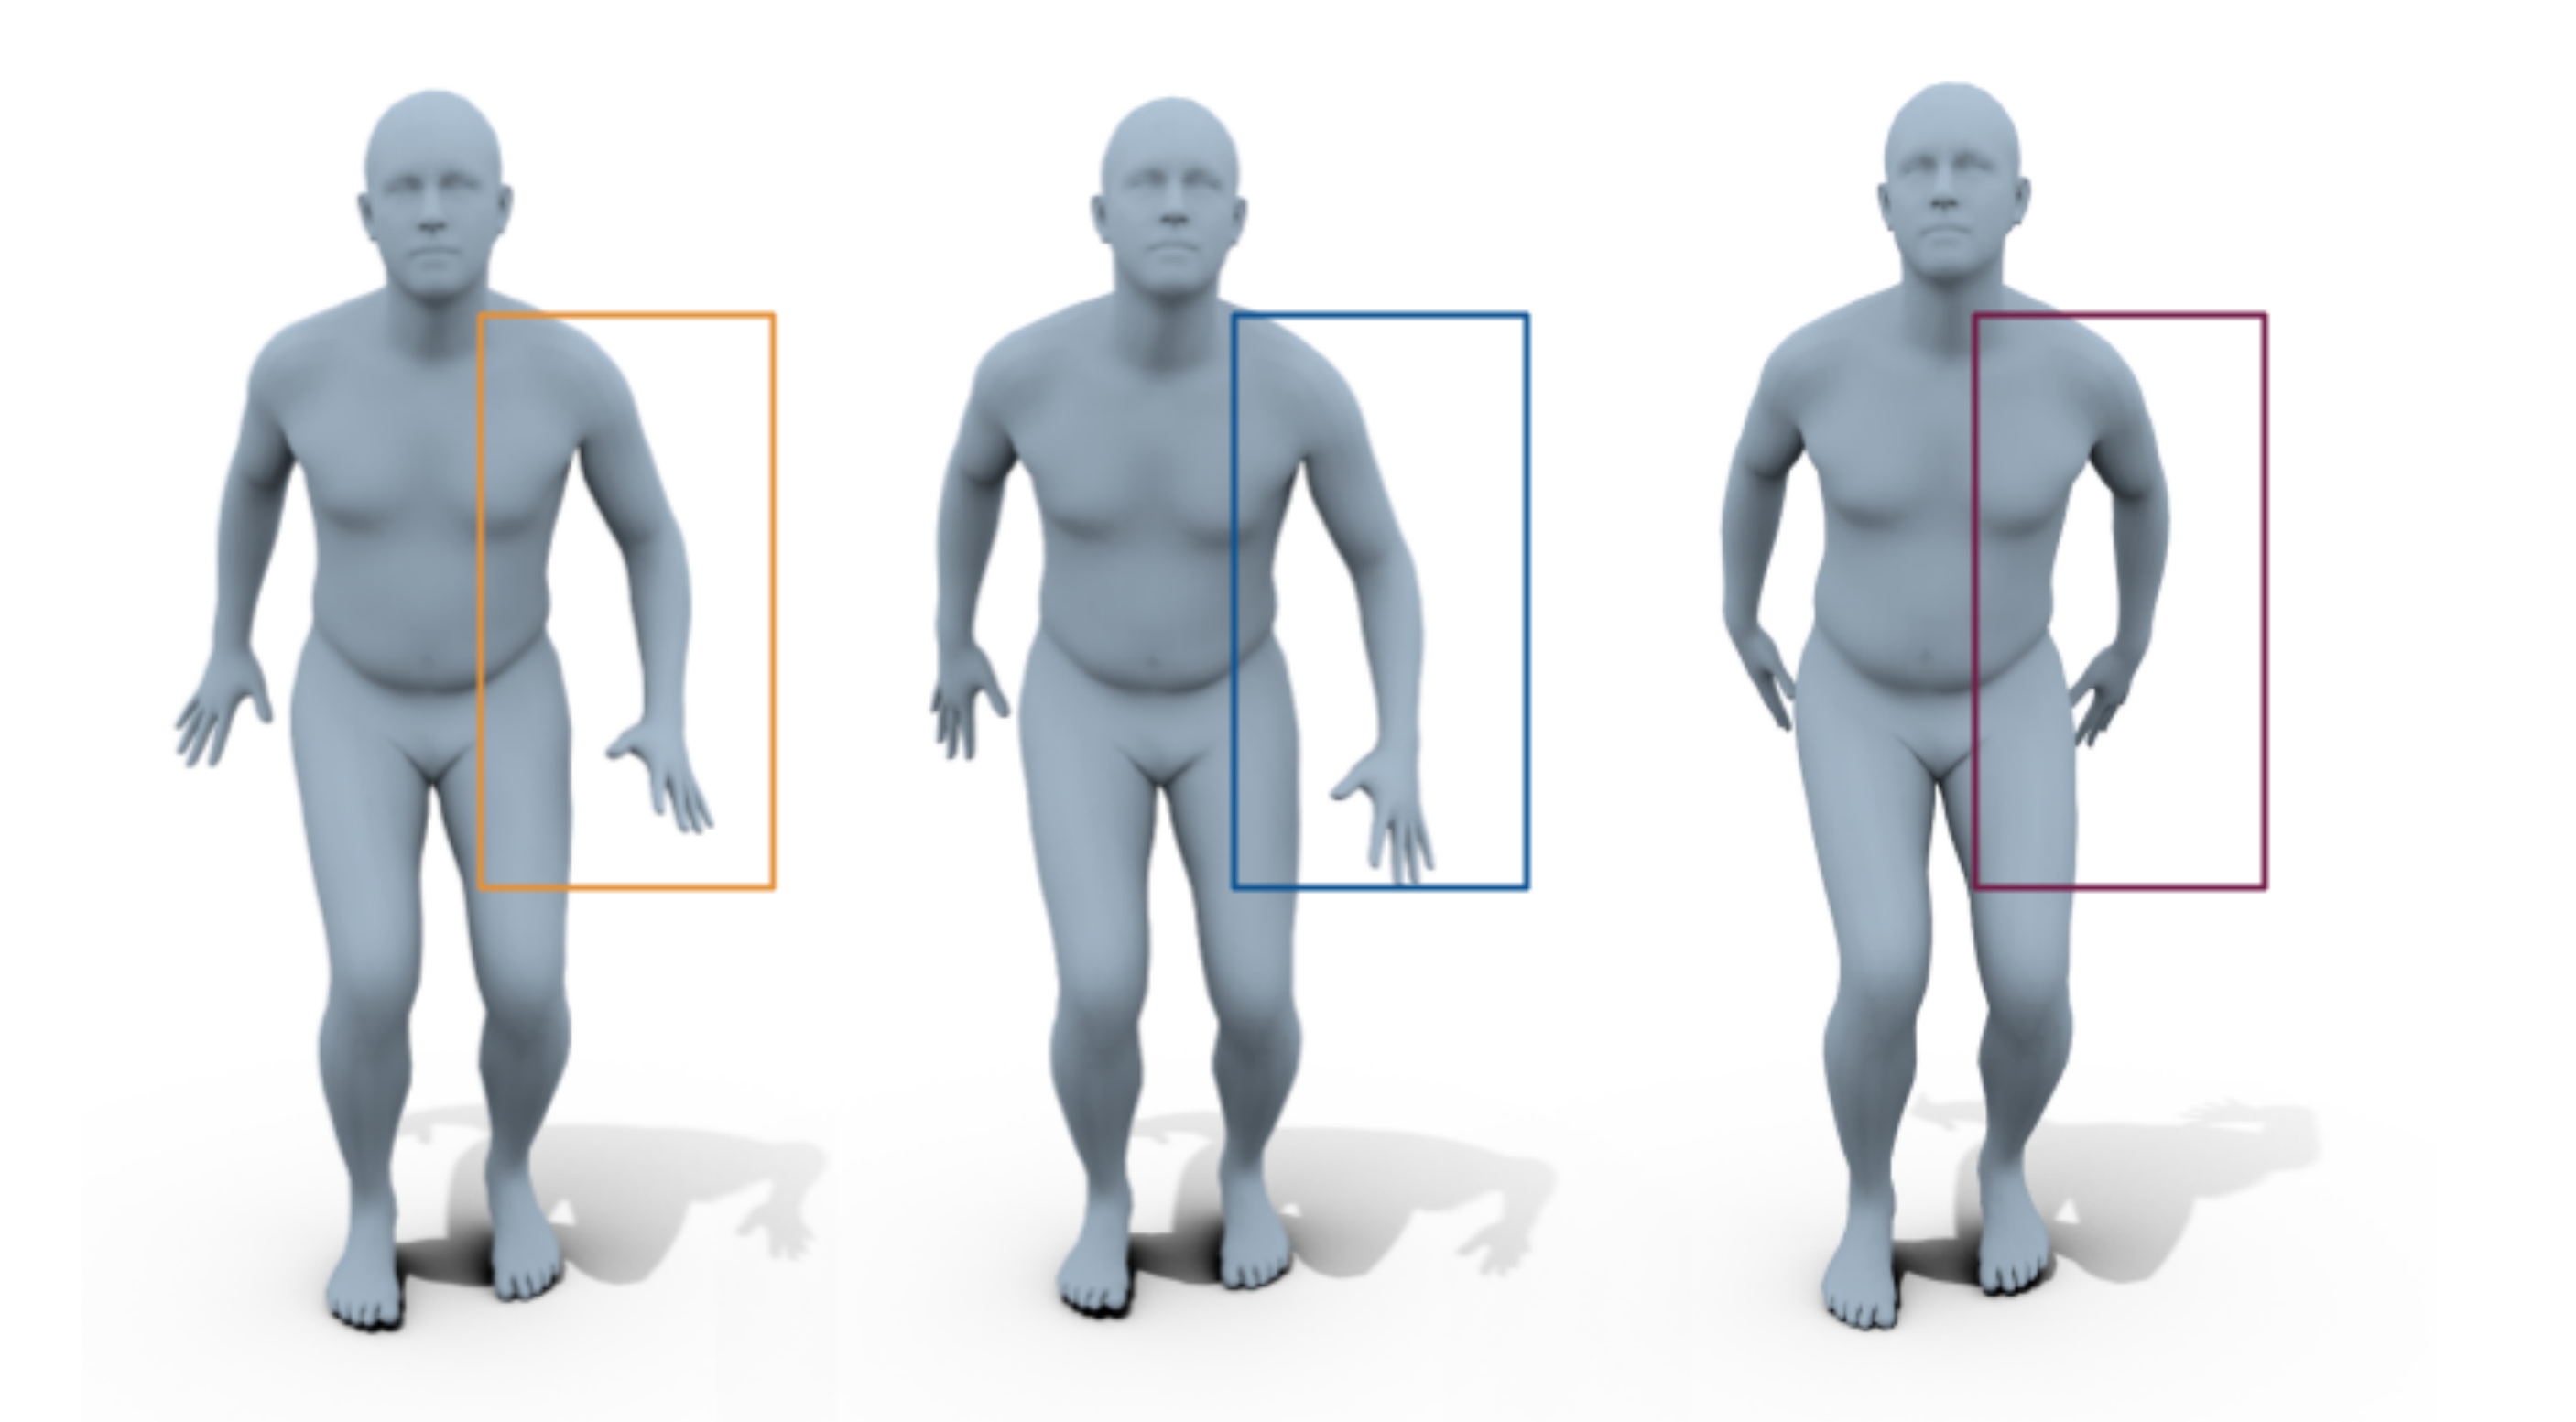}
     		\put(5,32){\colorbox{white}{\parbox{0.05\linewidth}{%
     \scriptsize{VPoser}}}}

  	    \put(25,32){\colorbox{white}{\parbox{0.05\linewidth}{%
     \scriptsize{HuMoR}}}}
       	    \put(42,32){\colorbox{white}{\parbox{0.05\linewidth}{%
     \scriptsize{Ours}}}}

\end{overpic}
&
				\begin{overpic}[width=0.48\textwidth,unit=1mm]{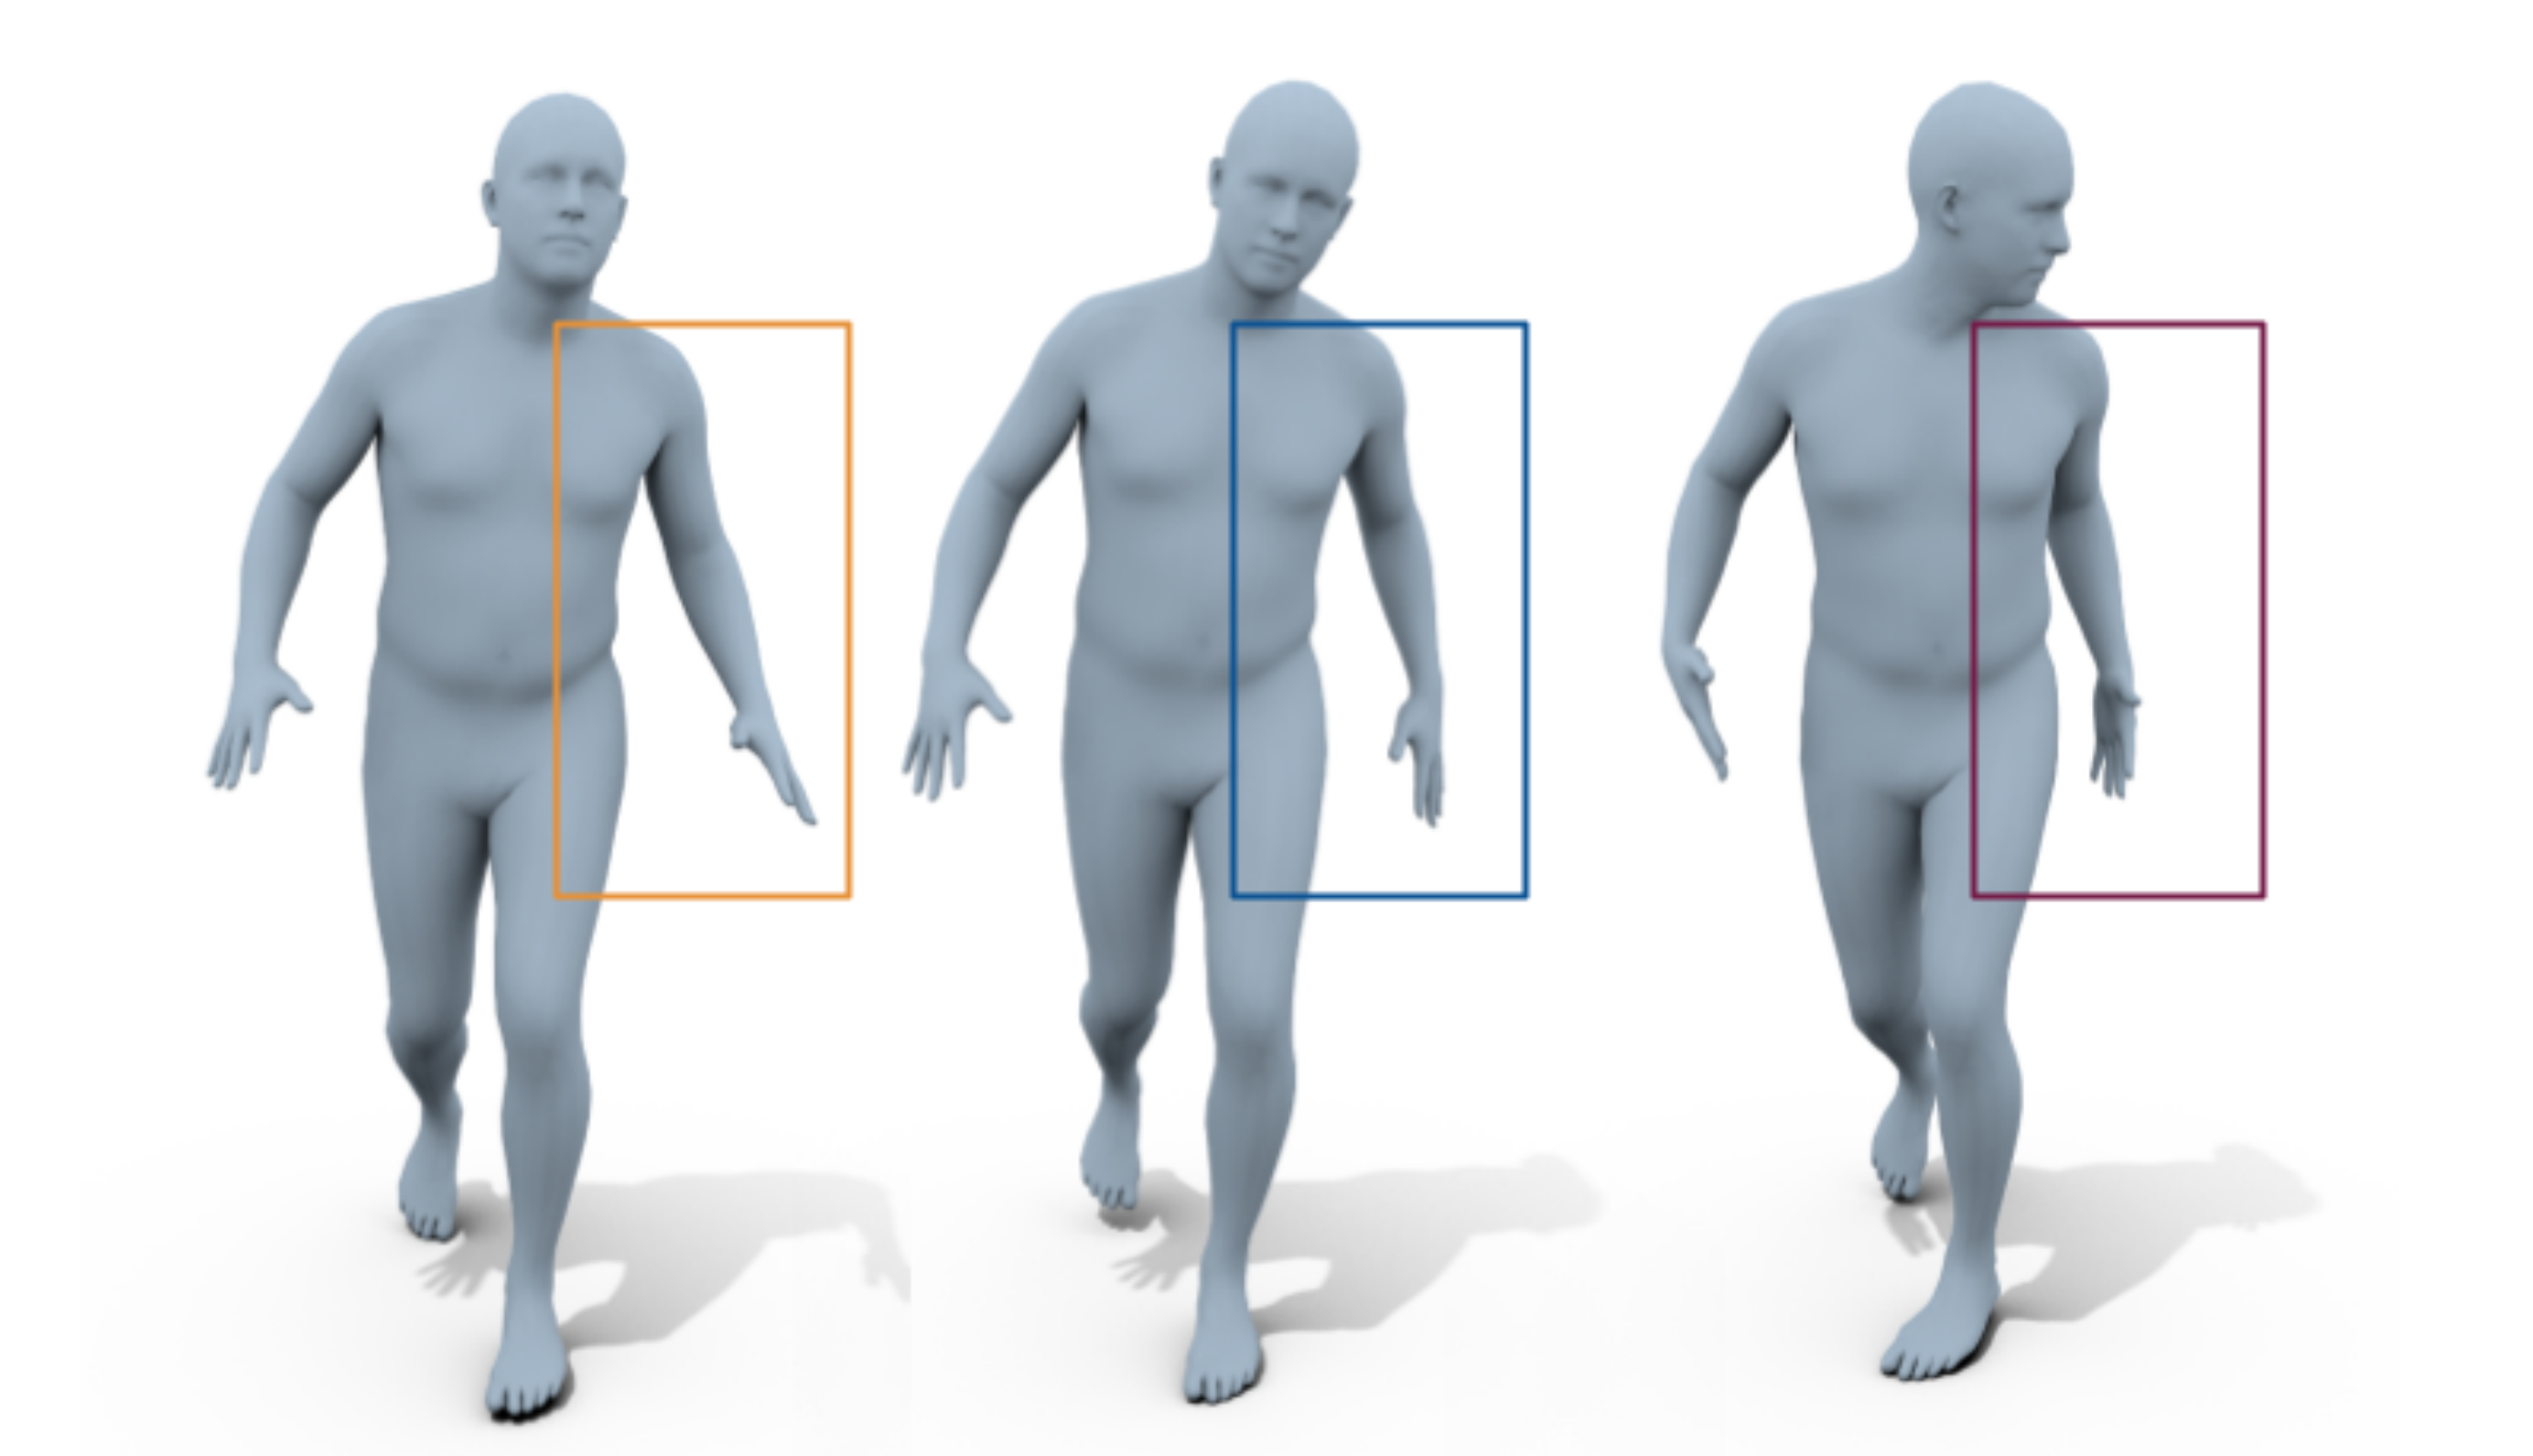}
     		\put(5,33){\colorbox{white}{\parbox{0.05\linewidth}{%
     \scriptsize{VPoser}}}}

  	    \put(25,33){\colorbox{white}{\parbox{0.05\linewidth}{%
     \scriptsize{HuMoR}}}}
       	    \put(42,33){\colorbox{white}{\parbox{0.05\linewidth}{%
     \scriptsize{Ours}}}}

\end{overpic}
\end{tabular}
	\caption{\textbf{Fitting to partial observation}: We compare VPoser, HuMoR and Pose-NDF based prior on the task of recovering 3D pose from partial observation. (Top): In case of occluded left leg, we observe that VPoser produces nearly straight legs(close to mean position), while HuMoR and PoseNDF produce much more diverse poses. HuMoR results in extreme unrealistic poses in some cases. We observe similar behavior for occluded arm case (bottom).}
	\label{fig:partial_suppl}
 	%\vspace{-0.5cm}
\end{figure}

\subsection{Pose Interpolation}
\label{sec:inter_suppl}

The \blah{} manifold can be used to interpolate between two distinct poses by traversing the manifold. We provide more such examples of pose interpolation using Pose-NDF in Fig~\ref{fig:inter_suppl}.

\begin{figure}[t]
	\centering
				\begin{overpic}[width=0.99\textwidth,unit=1mm]{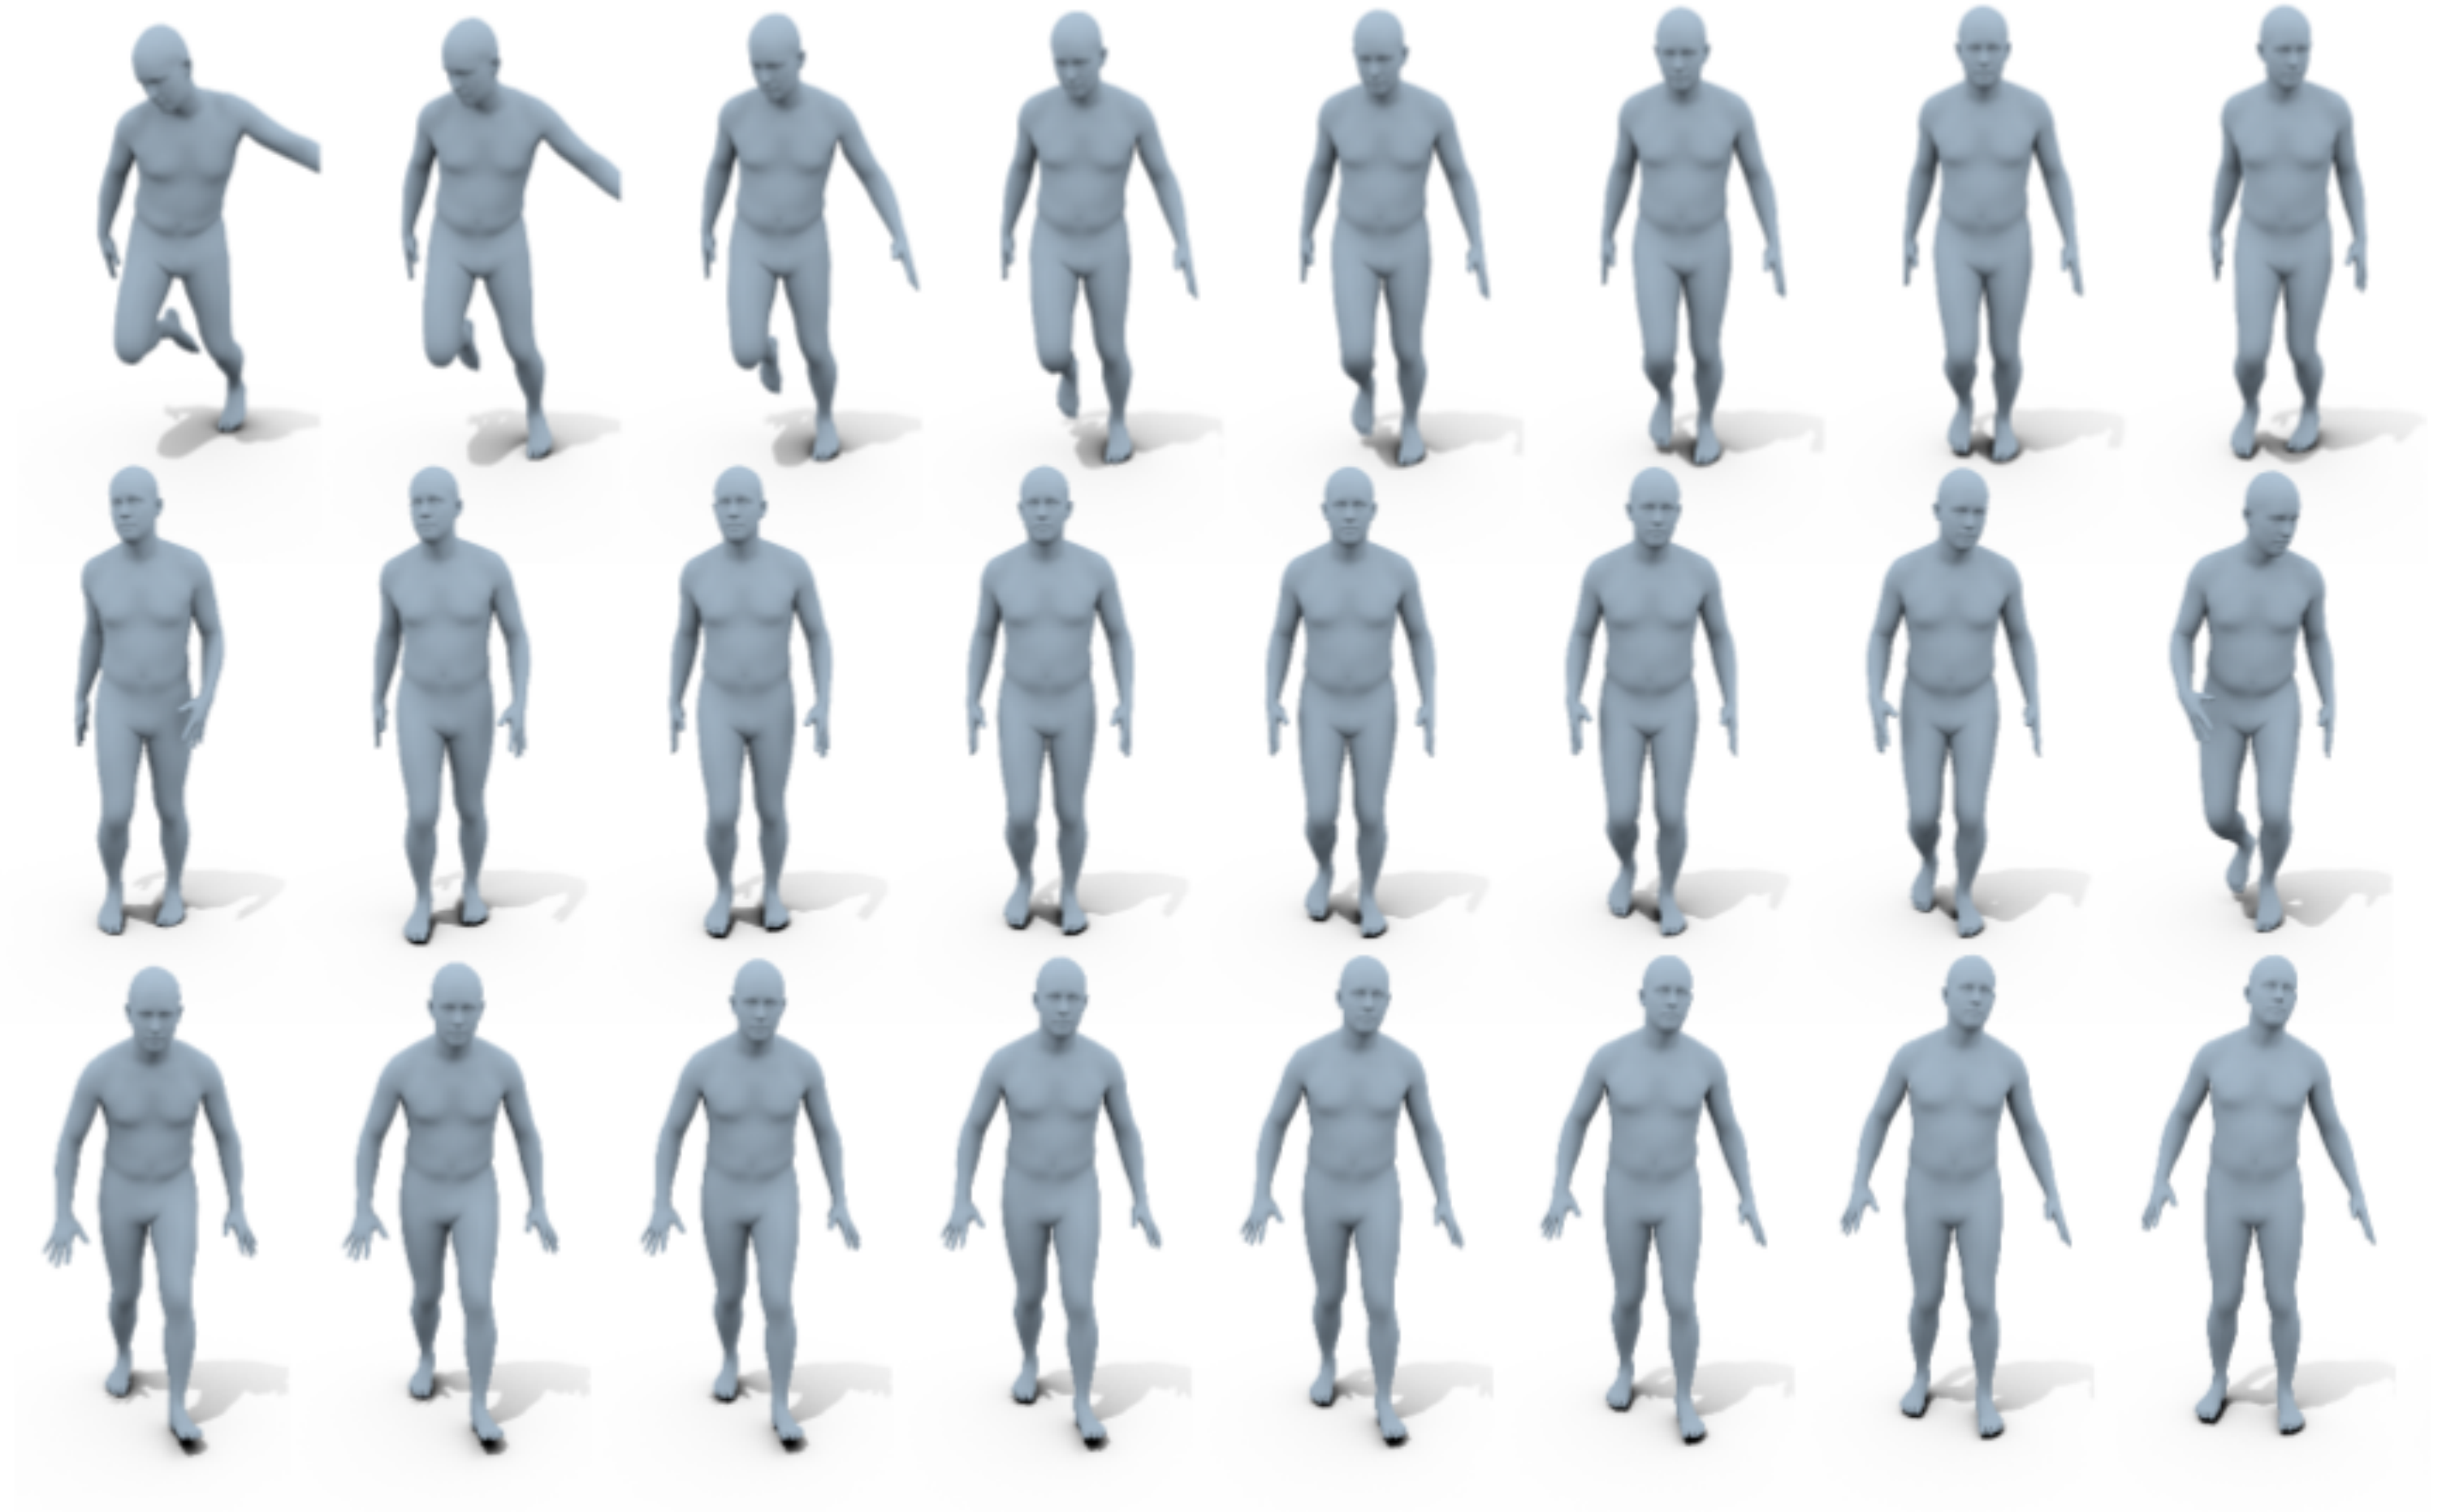}
     		\put(0,78){\colorbox{white}{\parbox{0.15\linewidth}{%
     \scriptsize{Start Pose}}}}
          		\put(105,78){\colorbox{white}{\parbox{0.15\linewidth}{%
     \scriptsize{End Pose}}}}
\end{overpic}

% 				\begin{overpic}[width=0.99\textwidth,unit=1mm]{images/interpolation/steps_6.pdf}

% \end{overpic}

	\caption{\textbf{Pose interpolation} using \blah{}.}
	\label{fig:inter_suppl}
\end{figure}

\subsection{Runtime}
\label{sec:runtime}
We compare the runtime of each method used in optimization based pose recovery methods. For motion denoising and motion recovery from partial observations, we conduct our experiments on a V100 GPU whereas for image based reconstruction, we used an RTX 3080Ti. HuMoR for motion denoising and pose recovery from partial observation takes approximately 10.83 sec. and 10.23 sec., respectively, for one frame. On the other hand, VPoser based optimization is way faster and takes only 0.96 sec. per frame. \blah{} based optimization takes even less: only 0.56 sec for motion denoising and partial observation experiments. This is because \blah{} is fast per step and has less optimization steps, as compared to VPoser and HuMoR. For the image based pose and shape reconstruction task, VPoser and \blah{}, take 3.63 sec. and 4.59 sec. respectively.
